# Supplementary material for: Predicting the Number of Future Events
Source: arXiv:2007.08648 source file (2020-08-07)
Supplement: Supplementary file 1 [file supplementary.pdf]

# Predicting the Number of Future Events: Supplementary Material

Qinglong Tian, Fanqi Meng, Daniel J. Nordman, William Q. Meeker

Department of Statistics, Iowa State University
Ames, IA 50011

August 7, 2020

Section A outlines algorithms for computing prediction bounds with the calibration-bootstrap method in the context of single-cohort and multiple-cohort within-sample prediction. Section B provides additional simulation results for Section 9.2 of the main paper, regarding a comparison of prediction bounds from direct/GPQ-bootstrap methods with limited failure time/event information. Proofs of the main results about the asymptotic coverage properties of prediction bound methods (Theorems 1-3 from the paper) are given in Section C; these concern the single-cohort case of within-sample prediction. Extensions of these proofs to handle the multiple-cohort case are discussed in Section D. The rest of the simulation results and the Bearing Cage Data are given in Section E. Section F provides some illustrative comparisons to show how the probabilities of future events in prediction may vary by distributional model.

# Section A Algorithms

Algorithm 1 describes the implementation of the calibration method with bootstrap Monte Carlo simulation. The procedure described in the main paper requires an extra layer of simulation (i.e., simulating $y^*$ from $\text{binom}(n - r_n^*, \widehat{p}_n)$). The algorithm described below avoids this extra layer of simulation thus reducing the Monte Carlo error. But as a trade-off, more memory space is needed.

---

**Algorithm 1:** Using Bootstrap Samples to Obtain the Calibrated Upper Prediction Bound

---

**Input:** The Type I censored single cohort data:$\boldsymbol{D}_n$; The bootstrap sample size: B; The nominal level:$1-\alpha$.

**Output:** The $100(1-\alpha)\%$ upper calibrated prediction bound:$\tilde{Y}^C_{n,1-\alpha}$.

compute estimators $\widehat{\boldsymbol{\theta}}_n = \widehat{\boldsymbol{\theta}}_n(\boldsymbol{D}_n)$ and $\widehat{p}_n = \pi(\widehat{\boldsymbol{\theta}}_n)$ (e.g., by maximum likelihood);

$b \leftarrow 1$;

$\text{values\_vector} \leftarrow \text{NULL}$; $\text{prob\_vector} \leftarrow \text{NULL}$;

**while** $b \leq B$ **do**

  simulate the $b$th bootstrap sample $\boldsymbol{D}_n^{*(b)}$; the number of failures in $\boldsymbol{D}_n^{*(b)}$ is $r_b^*$;

  compute $\widehat{\boldsymbol{\theta}}^*_b$, as the estimate of $\boldsymbol{\theta}$ from the bootstrap sample $\boldsymbol{D}_n^{*(b)}$;

  $\widehat{p}^*_b = \pi(\widehat{\boldsymbol{\theta}}^*_b)$, where $\pi(\cdot)$ is defined in (3);

  $\text{values\_vector} \leftarrow \mathbf{c}(\text{values\_vector}, \mathbf{pbinom}(0:(n-r_b^*), n-r_b^*, \widehat{p}^*_b))$;

  $\text{prob\_vector} \leftarrow \mathbf{c}(\text{prob\_vector}, \mathbf{dbinom}(0:(n-r_b^*), n-r_b^*, \widehat{p}_n))$;

  $b \leftarrow b+1$;

**end**

$\text{prob\_vector} \leftarrow \text{prob\_vector/B}$;

$\text{prob\_vector} \leftarrow \text{prob\_vector}[\mathbf{order}(\text{values\_vector})]$;

$\text{empirical\_cdf\_y} \leftarrow \mathbf{cumsum}(\text{prob\_vector})$;

$\text{empirical\_cdf\_x} \leftarrow \mathbf{sort}(\text{values\_vector})$;

$\text{p\_calibrated} \leftarrow \text{empirical\_cdf\_x}[\mathbf{which}(\text{empirical\_cdf\_y} \geq 1-\alpha)[1]]$;

$\tilde{Y}^C_{n,1-\alpha} \leftarrow \mathbf{qbinom}(\text{p\_calibrated}, n-r, \widehat{p}_n)$;

---

For multiple-cohort data, the only difference is that the binomial distribution is replaced a the Poisson-binomial distribution. Algorithm 2 provides an extension of Algorithm 1 for multiple-cohort data. The functions in bold correspond to the functions available in **R**. Again only results for the upper prediction bounds are given because results for the lower prediction

bounds are similar.

**Algorithm 2:** Extending **Algorithm** 1 to multiple-cohort Data

**Input:** The Type I censoring multiple-cohort data:$\mathbb{D}$; The bootstrap sample size: B; The nominal level:$1-\alpha$.

**Output:** The $100(1-\alpha)\%$ upper calibrated prediction bound:$\tilde{Y}^{C}_{n,1-\alpha}$.

compute the ML estimates $\widehat{\boldsymbol{\theta}}_n = \widehat{\boldsymbol{\theta}}_n(\mathbb{D})$ and $\widehat{\boldsymbol{p}}_n = (\pi_1(\widehat{\boldsymbol{\theta}}_n), ..., \pi_S(\widehat{\boldsymbol{\theta}}_n))$.
the numbers of remaining units are $\boldsymbol{w} = (n_1 - r_{n_1}, \ldots, n_S - r_{n_S})$;
$b \leftarrow 1$;
$\text{values\_vector} \leftarrow \text{NULL}; \text{prob\_vector} \leftarrow \text{NULL};$
**while** $b \leq B$ **do**
  simulate the $b$th bootstrap sample $\mathbb{D}^*_b$;
  the number of remaining units for each cohort in $\mathbb{D}^*_b$ is $\boldsymbol{w}^*_b = (n_1 - r^{*,b}_{n_1}, ..., n_S - r^{*,b}_{n_S})$;
  The total number of units at risk in the bootstrap sample $\mathbb{D}^*_b$ is $R_b = \sum_{s=1}^{S}(n_s - r^{*,b}_{n_s})$;
  compute $\widehat{\boldsymbol{\theta}}^*_b = \widehat{\boldsymbol{\theta}}^*_b(\mathbb{D}^*_b)$, the ML estimates of $\boldsymbol{\theta}$ from the bootstrap sample $\mathbb{D}^*_b$;
  compute $\widehat{\boldsymbol{p}}^*_b = (\pi_1(\widehat{\boldsymbol{\theta}}^*_b), ..., \pi_S(\widehat{\boldsymbol{\theta}}^*_b))$;
  $\text{values\_vector} \leftarrow \mathbf{c}(\text{values\_vector}, \mathbf{ppoibin}(0:R_b, \widehat{\boldsymbol{p}}^*_b, \boldsymbol{w}^*_b))$;
  $\text{prob\_vector} \leftarrow \mathbf{c}(\text{prob\_vector}, \mathbf{dpoibin}(0:R_b, \widehat{\boldsymbol{p}}_n, \boldsymbol{w}^*_b))$;
  $b \leftarrow b + 1$;
**end**
$\text{prob\_vector} \leftarrow \text{prob\_vector/B}$;
$\text{prob\_vector} \leftarrow \text{prob\_vector}[\mathbf{order}(\text{values\_vector})]$;
$\text{empirical\_cdf\_y} \leftarrow \mathbf{cumsum}(\text{prob\_vector})$;
$\text{empirical\_cdf\_x} \leftarrow \mathbf{sort}(\text{values\_vector})$;
$\text{p\_calibrated} \leftarrow \text{empirical\_cdf\_x}[\mathbf{which}(\text{empirical\_cdf\_y} \geq 1-\alpha)[1]]$;
$\tilde{Y}^{C}_{n,1-\alpha} \leftarrow \mathbf{qpoibin}(\text{p\_calibrated}, \widehat{\boldsymbol{p}}_n, \boldsymbol{w})$;

# Section B Comparing the Direct-Bootstrap and the GPQ-Bootstrap Methods

The numerical results presented here provide additional supporting details for the simulation study described in Section 9.2, intended to compare direct-bootstrap and GPQ-bootstrap methods for data with limited event information (e.g., few failures). Table 5 gives the prediction

bounds from 10 Monte Carlo samples using $d = 0.005$, where $d$ again denotes the (unconditional) probability of an event in a future window $(t_c, t_w]$ under the Weibull model. Figure 5

| Sample | Lower 95% | | Lower 90% | | Upper 90% | | Upper 95% | |
|---|---|---|---|---|---|---|---|---|
| | Direct | GPQ | Direct | GPQ | Direct | GPQ | Direct | GPQ |
| 1 | 5 | 4 | 9 | 6 | 360 | 164 | 975 | 392 |
| 2 | 4 | 3 | 7 | 5 | 222 | 115 | 574 | 254 |
| 3 | 0 | 0 | 0 | 0 | 13 | 12 | 17 | 18 |
| 4 | 17 | 11 | 29 | 18 | 3851 | 1390 | 4993 | 3188 |
| 5 | 6 | 5 | 10 | 7 | 374 | 164 | 1052 | 417 |
| 6 | 9 | 7 | 15 | 10 | 991 | 396 | 3367 | 986 |
| 7 | 5 | 3 | 8 | 6 | 315 | 152 | 970 | 308 |
| 8 | 14 | 9 | 22 | 14 | 2498 | 770 | 4934 | 1905 |
| 9 | 57 | 80 | 108 | 120 | 4956 | 4986 | 4997 | 4997 |
| 10 | 4 | 2 | 6 | 4 | 264 | 116 | 825 | 243 |

Table 5: Prediction Bounds of A Few Monte Carlo Samples.

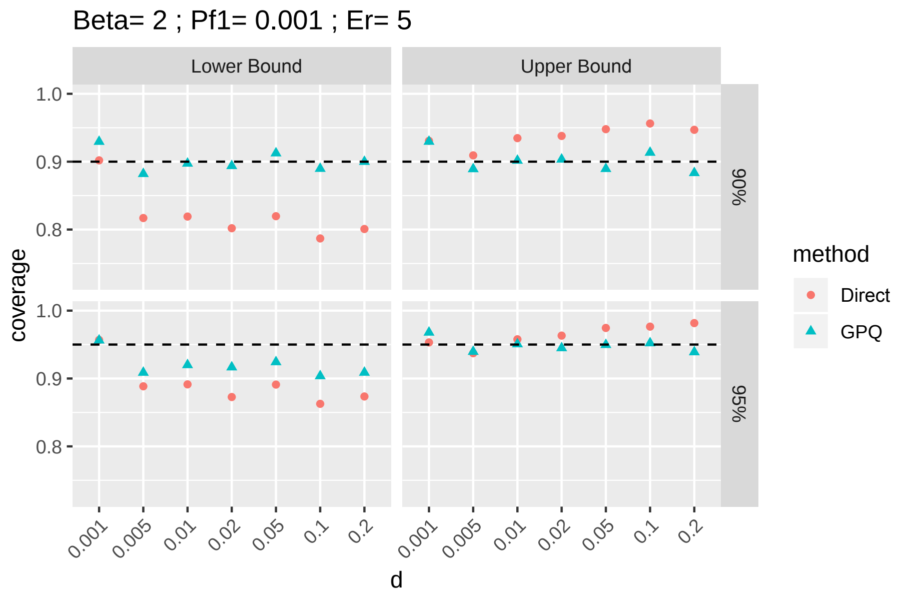


Figure 5: The Coverage Probabilities of the Direct-Bootstrap and GPQ-Bootstrap Methods.

shows the coverage probabilities of the direct-bootstrap and GPQ-bootstrap methods using different values of $d$. These results are referred to in the discussion of Section 9.2. Asymptotically,

both $\widehat{p}_n^*$ and $\widehat{p}_n^{**}$ are normally distributed and symmetric around $\widehat{p}_n$, as shown in Lemma 2 below.

# Section C Proof of the Theorems

Here we focus on the single-cohort version of the within-sample prediction problem and the corresponding Theorems 1-3 for the prediction bound methods. Extensions of these theorems to multiple-cohort data are then discussed in Section D. The proofs of the main results require three technical lemmas (Lemmas 1-3) given next; after establishing these lemmas, proofs of Theorems 1-3 are then provided.

Recall that, under the conditions for Theorem 1, the parameter estimators $\widehat{\boldsymbol{\theta}}_n \in \mathbb{R}^q$ (e.g., ML estimators) have a normal limit, i.e., $\sqrt{n}(\widehat{\boldsymbol{\theta}}_n - \boldsymbol{\theta}_0)$ converges in distribution to a multivariate normal $\mathrm{MVN}(\mathbf{0}, \boldsymbol{V}_0)$. For later reference, Lemma 1 states that the bootstrap version of parameter estimators, given by $\sqrt{n}(\widehat{\boldsymbol{\theta}}_n^* - \widehat{\boldsymbol{\theta}}_n)$ (e.g., as generated by a parametric bootstrap), has the same normal limit under the mild consistency assumptions of Theorem 2.

**Lemma 1.** *Suppose conditions from Theorem 2. Letting $\mathcal{L}_n^*$ denote the bootstrap probability distribution of $\sqrt{n}(\widehat{\boldsymbol{\theta}}_n^* - \widehat{\boldsymbol{\theta}}_n)$ and letting $\mathcal{L}$ denote the $\mathrm{MVN}(\mathbf{0}, \boldsymbol{V}_0)$ probability distribution, the distance $\rho(\mathcal{L}_n^*, \mathcal{L})$ between these distributions satisfies*

$$\rho(\mathcal{L}_n^*, \mathcal{L}) \xrightarrow{p} 0, \textit{as } n \to \infty,$$

*under any distance $\rho(\cdot,\cdot)$ (e.g., Prokhorov distance) which metricizes weak convergence on $\mathbb{R}^q$.*

*Proof.* If $\mathcal{L}_n$ denotes the sampling distribution of $\sqrt{n}(\widehat{\boldsymbol{\theta}}_n - \boldsymbol{\theta}_0)$, then the Theorem 1-2 conditions give $\rho(\mathcal{L}_n, \mathcal{L}) \to 0$ and $\rho(\mathcal{L}_n^*, \mathcal{L}_n) \xrightarrow{p} 0$ (by assumption). By the triangle inequality ($\rho$ is a metric), $\rho(\mathcal{L}_n^*, \mathcal{L}) \leq \rho(\mathcal{L}_n^*, \mathcal{L}_n) + \rho(\mathcal{L}_n, \mathcal{L}) \xrightarrow{p} 0$. □

Lemma 2 next establishes certain normal limits for estimators of the conditional probability $p = \pi(\theta)$ from (3), at both the original data and bootstrap levels. Lemma 2 implies that the

bootstrap counterparts of $\sqrt{n}(\widehat{p}_n - p_0)$ converge in distribution to the same normal limit $N(0, v_0)$ as the estimator $\widehat{p}_n$ does.

**Lemma 2.** *Let* $v_0 \equiv \nabla_0^t \boldsymbol{V}_0 \nabla_0 > 0$ *with* $\boldsymbol{V}_0$ *and non-zero* $\nabla_0 = \partial\pi(\boldsymbol{\theta})/\partial\boldsymbol{\theta}|_{\boldsymbol{\theta}=\boldsymbol{\theta}_0}$ *from Theorem 1, where* $\boldsymbol{\theta}_0$ *contains the true parameters and* $\pi(\cdot)$ *is from (3). Let* $\Phi_{\mathrm{nor}}(z/\sqrt{v_0})$*,* $z \in \mathbb{R}$*, denote the cdf of a normal* $N(0, v_0)$ *(*$v_0$ *is the variance). Then under Theorem 2 conditions, as* $n \to \infty$*,*

*(1)* $\sqrt{n}(\widehat{p}_n - p_0) \xrightarrow{d} N(0, v_0)$ *holds for the estimator* $\widehat{p}_n = \pi(\widehat{\boldsymbol{\theta}}_n)$ *of* $p_0 = \pi(\boldsymbol{\theta}_0)$*.*

*(2) In the direct-bootstrap method, for the bootstrap version* $\sqrt{n}(\widehat{p}_n^* - \widehat{p}_n)$ *of* $\sqrt{n}(\widehat{p}_n - p_0)$*, it holds that*

$$\sup_{z\in\mathbb{R}} \left|\Pr_*(\sqrt{n}(\widehat{p}_n^* - \widehat{p}_n) \le z) - \Phi_{\mathrm{nor}}(z/\sqrt{v_0})\right| \xrightarrow{p} 0.$$

*(3) In the GPQ-bootstrap method where* $F(\cdot; \mu_0, \sigma_0)$ *belongs to the log-location-scale family, for the approximate GPQ-based bootstrap version of* $\sqrt{n}(\widehat{p}_n - p_0)$*, it holds that*

$$\sup_{z\in\mathbb{R}} \left|\Pr_*(\sqrt{n}(\widehat{p}_n^{**} - \widehat{p}_n) \le z) - \Phi_{\mathrm{nor}}(z/\sqrt{v_0})\right| \xrightarrow{p} 0.$$

*Proof.* Part 1 of Lemma 2 follows from the normal limit for $\sqrt{n}(\widehat{\boldsymbol{\theta}}_n - \boldsymbol{\theta})$ assumed in Theorem 1 along with the delta method as the parametric function $p = \pi(\boldsymbol{\theta})$ is differentiable at $\boldsymbol{\theta}_0$. The positivity of $v_0$ follows because the matrix $\boldsymbol{V}_0$ is positive definite and the vector $\nabla_0$ is non-zero.

To show the convergence in probability stated in Part 2 of Lemma 2, we use the characterization of convergence in probability through almost sure convergence along subsequences. Let $\{n_j\} \subset \{n\}$ be an arbitrary subsequence of indices. Since $\widehat{\boldsymbol{\theta}}_n \xrightarrow{p} \boldsymbol{\theta}_0$ under Theorem 1 and $\rho(\mathcal{L}_n^*, \mathcal{L}) \xrightarrow{p} 0$ by Lemma 1, there exists a further subsequence $\{n_k\} \subset \{n_j\}$ and both $\widehat{\boldsymbol{\theta}}_{n_k} \to \boldsymbol{\theta}_0$ and $\rho(\mathcal{L}_{n_k}^*, \mathcal{L}_{n_k}) \to 0$ converge almost surely. That is, associating the original random variables with a probability space $(\Omega, \mathscr{F}, P)$ involving a sample space $\Omega$ and the associated $\sigma$-algebra $\mathscr{F}$ of events, there exists an event $A \in \mathscr{F}$ with $P(A) = 1$ such that, for any sample point

$\omega \in A$, it holds that $\widehat{\boldsymbol{\theta}}_{n_k} \equiv \widehat{\boldsymbol{\theta}}_{n_k}(\omega) \to \boldsymbol{\theta}_0$ and $\rho(\mathcal{L}^*_{n_k}, \mathcal{L}) \equiv \rho(\mathcal{L}^*_{n_k}, \mathcal{L})(\omega) \to 0$ as $n_k \to \infty$ (i.e., pointwise convergence at each $\omega \in A$ along the subsequence $\{n_k\}$). Note that, given $\omega \in A$, estimates $\widehat{\boldsymbol{\theta}}_{n_k}(\omega)$ correspond to a single real sequence and there is a single sequence of bootstrap distributions $\mathcal{L}^*_{n_k}$, $n_k \geq 1$, for the bootstrap estimators $\sqrt{n_k}(\widehat{\boldsymbol{\theta}}^*_{n_k} - \widehat{\boldsymbol{\theta}}_{n_k}(\omega))$ induced by the bootstrap probability $\Pr_*$. To simplify the notation, we shall fix $\omega \in A$ and consider pointwise convergence at $\omega \in A$ as $n_k \to \infty$, suppressing the appearance of $\omega$ in the notation. Standard convergence in probability or distribution, though, with respect to the bootstrap probability $\Pr_*$ along the subsequence $\{n_k\}$, will be denoted as $\xrightarrow{d^*}$ and $\xrightarrow{p^*}$, respectively, for clarity. Hence along the subsequence $\{n_k\}$, it holds that $\widehat{\boldsymbol{\theta}}_{n_k} \to \boldsymbol{\theta}_0$ and $\sqrt{n_k}(\widehat{\boldsymbol{\theta}}^*_{n_k} - \widehat{\boldsymbol{\theta}}_{n_k}(\omega)) \xrightarrow{d^*} \boldsymbol{Z}_2$ for the multivariate normal random vector $\boldsymbol{Z}_2 \sim N(\boldsymbol{0}, \boldsymbol{V}_0)$ from Lemma 1.

We next define $\nabla(\boldsymbol{\theta}) = \partial\pi(\boldsymbol{\theta})/\partial\boldsymbol{\theta}$, which is assumed to exist in a neighborhood of $\boldsymbol{\theta}_0$. Note that $\widehat{\boldsymbol{\theta}}^*_{n_k} \overset{p*}{\to} \boldsymbol{\theta}_0$ follows by $\widehat{\boldsymbol{\theta}}^*_{n_k} - \widehat{\boldsymbol{\theta}}_{n_k} \overset{p*}{\to} 0$ and $\widehat{\boldsymbol{\theta}}_{n_k} \to \boldsymbol{\theta}_0$. Consequently, for $\widehat{p}^*_{n_k} = \pi(\widehat{\boldsymbol{\theta}}^*_{n_k})$ and $\widehat{p}_{n_k} = \pi(\widehat{\boldsymbol{\theta}}_{n_k})$ based on the (continuously differentiable near $\boldsymbol{\theta}_0$) parametric function $\pi(\cdot)$ in (3), we use a Taylor expansion of $\pi(\widehat{\boldsymbol{\theta}}^*_{n_k})$ around $\widehat{\boldsymbol{\theta}}_{n_k}$ to obtain

$$\sqrt{n_k}(\widehat{p}^*_{n_k} - \widehat{p}_{n_k}) = \left[\nabla(\boldsymbol{c}^*_{n_k})\right]^t \sqrt{n_k}(\widehat{\boldsymbol{\theta}}^*_{n_k} - \widehat{\boldsymbol{\theta}}_{n_k}),$$

where $\nabla(\boldsymbol{c}^*_{n_k})$ is the gradient $\nabla(\boldsymbol{\theta})$ evaluated at $\boldsymbol{c}^*_{n_k} = \alpha^*_{n_k}\widehat{\boldsymbol{\theta}}_{n_k} + (1-\alpha^*_{n_k})\widehat{\boldsymbol{\theta}}^*_{n_k}$ for some $\alpha^*_{n_k} \in [0,1]$. Because $\widehat{\boldsymbol{\theta}}_{n_k} \to \boldsymbol{\theta}_0$ and $\widehat{\boldsymbol{\theta}}^*_{n_k} \xrightarrow{p^*} \widehat{\boldsymbol{\theta}}_{n_k}$, we have

$$\begin{aligned}
\|\boldsymbol{c}^*_{n_k} - \boldsymbol{\theta}_0\| &= \|\alpha^*_{n_k}(\widehat{\boldsymbol{\theta}}_{n_k} - \boldsymbol{\theta}_0) + (1-\alpha^*_{n_k})(\widehat{\boldsymbol{\theta}}^*_{n_k} - \boldsymbol{\theta}_0)\| \\
&\leq \|\alpha^*_{n_k}(\widehat{\boldsymbol{\theta}}_{n_k} - \boldsymbol{\theta}_0)\| + \|(1-\alpha^*_{n_k})(\widehat{\boldsymbol{\theta}}^*_{n_k} - \widehat{\boldsymbol{\theta}}_{n_k})\| + \|((1-\alpha^*_{n_k})(\widehat{\boldsymbol{\theta}}_{n_k} - \boldsymbol{\theta}_0)\| \\
&\leq 2\|\widehat{\boldsymbol{\theta}}_{n_k} - \boldsymbol{\theta}_0\| + \|\widehat{\boldsymbol{\theta}}^*_{n_k} - \widehat{\boldsymbol{\theta}}_{n_k}\| \xrightarrow{p^*} 0
\end{aligned}$$

as $n_k \to \infty$. Because $\nabla(\boldsymbol{\theta})$ is continuous at $\boldsymbol{\theta}_0$, the continuous mapping theorem then gives

$$\nabla(\boldsymbol{c}^*_{n_k}) \xrightarrow{p^*} \nabla(\boldsymbol{\theta}_0) \equiv \nabla_0$$

and then Slutsky's theorem yields $\sqrt{n_k}(\widehat{p}^*_{n_k} - \widehat{p}_{n_k}) \xrightarrow{d^*} \nabla_0^t \boldsymbol{Z}_2$. Because the random variable $\nabla_0^t \boldsymbol{Z}_2$ is continuous with cdf $\Phi_{\text{nor}}(z/\sqrt{v_0})$, $z \in \mathbb{R}$, Polya's theorem then implies uniform convergence of cdfs as

$$\sup_{z\in\mathbb{R}} \left|\Pr_*(\sqrt{n_k}(\widehat{p}^*_{n_k} - \widehat{p}_{n_k}) \leq z) - \Phi_{\text{nor}}(z/\sqrt{v_0})\right| \to 0$$

as $n_k \to \infty$. Because the above distance between distributions converges almost surely to zero along the subsequence $\{n_k\} \subset \{n_j\}$ and because the subsequence $\{n_j\}$ was arbitrary, we have shown that every subsequence contains a further subsequence where this distributional distance converges to zero almost surely; the probabilistic convergence in Part 2 of Lemma 2 then follows.

For the GPQ-bootstrap method in Part 3 of Lemma 2, we define $h(z, x, y) = \Phi\left[z(1 + y/\widehat{\sigma}_{n_k}) + x/\widehat{\sigma}_{n_k}\right]$, $\widehat{z}_w = [\log(t_w) - \widehat{\mu}_{n_k}]/\widehat{\sigma}_{n_k}$ and $\widehat{z}_c = [\log(t_c) - \widehat{\mu}_{n_k}]/\widehat{\sigma}_{n_k}$. Here $\Phi(\cdot) = F(\cdot; 0, 1)$ is the standard cdf of the log-location-scale distribution with derivative $\Phi'(\cdot) \equiv \phi(\cdot)$ on $\mathbb{R}$, and $\widehat{\mu}_{n_k}, \widehat{\sigma}_{n_k}$ are the consistent estimators of $\mu$ and $\sigma$. Then we define $g_n(x, y) = \left[h(\widehat{z}_w, x, y) - h(\widehat{z}_c, x, y)\right]/[1 - h(\widehat{z}_c, x, y)]$, so that $\widehat{p}^{**}_{n_k} - \widehat{p}_{n_k} = g_n(\widehat{\mu}^*_{n_k} - \widehat{\mu}_{n_k}, \widehat{\sigma}^*_{n_k} - \widehat{\sigma}_{n_k}) - g_n(0, 0)$. We use a Taylor expansion of $g_n(\widehat{\mu}^*_{n_k} - \widehat{\mu}_{n_k}, \widehat{\sigma}^*_{n_k} - \widehat{\sigma}_{n_k})$ at $(0, 0)$ to obtain

$$\sqrt{n_k}(\widehat{p}^{**}_{n_k} - \widehat{p}_{n_k}) = \left[(\partial g_n/\partial x, \partial g_n/\partial y)|_{x=0,y=0} + R^*_n\right] \sqrt{n_k}\left(\widehat{\mu}^*_{n_k} - \widehat{\mu}_{n_k}, \widehat{\sigma}^*_{n_k} - \widehat{\sigma}_{n_k}\right)^t,$$

where $R_n \xrightarrow{p*} 0$ by the differentiability of $g_n(x, y)$ at $(0, 0)$ combined with $\sqrt{n}(\widehat{\mu}^*_{n_k} - \widehat{\mu}_{n_k}, \widehat{\sigma}^*_{n_k} - \widehat{\sigma}_{n_k}) \xrightarrow{p*} 0$ and $(\widehat{\mu}_{n_k}, \widehat{\sigma}_{n_k}) \to (\mu_0, \sigma_0)$.

Because $(\widehat{\mu}_{n_k}, \widehat{\sigma}_{n_k}) \to (\mu_0, \sigma_0)$ and $R_n \xrightarrow{p} 0$ as $n_k \to \infty$, we have

$$\begin{aligned}\left(\frac{\partial g_n}{\partial x}, \frac{\partial g_n}{\partial y}\right)^t\Bigg|_{x=0,y=0} &\xrightarrow{p^*} \begin{pmatrix} \frac{1}{\sigma[1-\phi(z_c)]^2}\left\{\phi(z_c)[1 - \Phi(z_w)] - \phi(z_w)[1 - \Phi(z_c)]\right\} \\ \frac{1}{\sigma[1-\phi(z_c)]^2}\left\{z_c\phi(z_c)[1 - \Phi(z_w)] - z_w\phi(z_w)[1 - \Phi(z_c)]\right\} \end{pmatrix} \\ &= \left(\frac{\partial \pi(\mu, \sigma)}{\partial \mu}, \frac{\partial \pi(\mu, \sigma)}{\partial \sigma}\right)^t\Bigg|_{\mu=\mu_0,\sigma=\sigma_0} = \nabla_0,\end{aligned}$$

where we define $z_c = [\log(t_c) - \mu_0]/\sigma_0$, $z_w = [\log(t_w) - \mu_0]/\sigma_0$ and $\phi(\cdot)$ is the pdf/derivative of $\Phi(\cdot)$. The rest of the proof follows by Slutsky's theorem in the same manner as the proof for the direct-bootstrap method. $\square$

**Lemma 3.** *Let $Z_0$ and $Z_1$ denote independent standard normal random variables. Under the conditions for Theorem 1 conditions with true parameters $\boldsymbol{\theta}_0$, the following (1)-(3) hold as $n \to \infty$*

*(1)*

$$\frac{Y_n - (n - r_n)\widehat{p}_n}{\sqrt{(n - r_n)\widehat{p}_n(1 - \widehat{p}_n)}} \xrightarrow{d} Z_0 + \sqrt{v_1} Z_1,$$

*where $v_1 = v_0[1 - F(t_c; \boldsymbol{\theta}_0)]/[p_0(1 - p_0)]$ for $p_0 = \pi(\boldsymbol{\theta}_0)$ and $v_0$ is from Lemma 2.*

*(2) Based on the bootstrap version $\widehat{p}_n^* = \pi(\widehat{\boldsymbol{\theta}}_n^*)$ of $\widehat{p}_n = \pi(\widehat{\boldsymbol{\theta}}_n)$, let the random variable $Y_n^*$ be defined as $Y_n^* | \widehat{p}_n^* \sim \mathrm{Binomial}(n - r_n, \widehat{p}_n^*)$, where $r_n$ is the number of events in the given sample. Then it holds that*

$$\sup_{z \in \mathbb{R}} \left| \mathrm{Pr}_* \left[ \frac{Y_n^* - (n - r_n)\widehat{p}_n}{\sqrt{(n - r_n)\widehat{p}_n(1 - \widehat{p}_n)}} \leq z \right] - \Pr(Z_0 + \sqrt{v_1} Z_1 \leq z) \right| \xrightarrow{p} 0.$$

*(3) Based on the approximate GPQ-based bootstrap version $\widehat{p}_n^{**} = \pi(\widehat{\mu}_n^{**}, \widehat{\sigma}_n^{**})$ of $\widehat{p}_n = \pi(\widehat{\mu}_n, \widehat{\sigma}_n)$ and a random variable $Y_n^{**}$ defined as $Y_n^{**} | \widehat{p}_n^{**} \sim \mathrm{Binomial}(n - r_n, \widehat{p}_n^{**})$, it holds that*

$$\sup_{z \in \mathbb{R}} \left| \mathrm{Pr}_* \left[ \frac{Y_n^{**} - (n - r_n)\widehat{p}_n}{\sqrt{(n - r_n)\widehat{p}_n(1 - \widehat{p}_n)}} \leq z \right] - \Pr(Z_0 + \sqrt{v_1} Z_1 \leq z) \right| \xrightarrow{p} 0.$$

*Proof.* Fix $z \in \mathbb{R}$, based on the censored sample $\boldsymbol{D}_n$, define an event $M_n = M_{1n} \cap M_{2n}$, where $M_{1n} = \{r_n < n\}$ and $M_{2n} = \{0 < \widehat{p}_n < 1\}$. As $n \to \infty$, note that $\Pr(M_{2n}^c) \to 0$ by Lemma 2 Part 1 with $p_0 \in (0, 1)$ (cf. Theorem 1), while $\Pr(M_{1n}^c) = \Pr(r_n = n) = [F(t_c; \boldsymbol{\theta}_0)]^n \to 0$ (i.e., $F(t_c; \boldsymbol{\theta}_0) \in (0, 1)$ under Theorem 1 conditions). Hence, it follows that $\Pr(M_n) \to 1$ as $n \to \infty$ and the predictive root $[Y_n - (n - r_n)\widehat{p}_n] / \sqrt{(n - r_n)\widehat{p}_n(1 - \widehat{p}_n)}$ is well defined when the event $M_n$ holds. Hence, for fixed $z \in \mathbb{R}$, we may write

$$\left| \Pr \left[ \frac{Y_n - (n - r_n)\widehat{p}_n}{\sqrt{(n - r_n)\widehat{p}_n(1 - \widehat{p}_n)}} \leq z \right] - \tau_n \right| \leq \Pr(M_n^c) \to 0 \tag{C.1}$$

for

$$\tau_n \equiv \Pr\left[M_n, \frac{Y_n - (n-r_n)\widehat{p}_n}{\sqrt{(n-r_n)\widehat{p}_n(1-\widehat{p}_n)}} \le z\right]$$
$$= \Pr\left[M_n, \frac{Y_n - (n-r_n)p_0}{\sqrt{(n-r_n)p_0(1-p_0)}} \le z\frac{\sqrt{\widehat{p}_n(1-\widehat{p}_n)}}{\sqrt{p_0(1-p_0)}} + \frac{\sqrt{n-r_n}(\widehat{p}_n - p_0)}{\sqrt{p_0(1-p_0)}}\right].$$

Conditioning on the censored data $\boldsymbol{D}_n$, we further write a conditional probability version of $\tau_n$ as

$$\Pr\left[M_n, \frac{Y_n - (n-r_n)\widehat{p}_n}{\sqrt{(n-r_n)\widehat{p}_n(1-\widehat{p}_n)}} \le z \middle| \boldsymbol{D}_n\right]$$
$$= \mathrm{I}(M_n)\Pr\left[\frac{Y_n - (n-r_n)p_0}{\sqrt{(n-r_n)p_0(1-p_0)}} \le z\frac{\sqrt{\widehat{p}_n(1-\widehat{p}_n)}}{\sqrt{p_0(1-p_0)}} + \frac{\sqrt{n-r_n}(\widehat{p}_n - p_0)}{\sqrt{p_0(1-p_0)}} \middle| \boldsymbol{D}_n\right]$$
$$= \mathrm{I}(M_n)\Phi_{\text{nor}}\left[z\frac{\sqrt{\widehat{p}_n(1-\widehat{p}_n)}}{\sqrt{p_0(1-p_0)}} + \frac{\sqrt{n-r_n}(\widehat{p}_n - p_0)}{\sqrt{p_0(1-p_0)}}\right] + \mathrm{I}(M_n)R_n$$

where $\Phi_{\text{nor}}(\cdot)$ denotes a standard normal cdf, $\mathrm{I}(\cdot)$ denotes the indicator function, and $R_n$ is a remainder that satisfies

$$|R_n| \le \frac{1}{\sqrt{(n-r_n)p_0(1-p_0)}}$$

by the Berry-Esseen theorem applied to $(n-r_n)$ independent Bernoulli($p_0$) random variables. As $n \to \infty$, note that $(n-r_n)/n \xrightarrow{p} 1 - F(t_c;\boldsymbol{\theta}_0)$ by the weak law of large numbers, so that $R_n \xrightarrow{p} 0$ follows as well as

$$\frac{\sqrt{n-r_n}(\widehat{p}_n - p_0)}{\sqrt{p_0(1-p_0)}} = \frac{[(n-r_n)/n]^{1/2}}{\sqrt{p_0(1-p_0)}}\sqrt{n}(\widehat{p}_n - p_0) \xrightarrow{d} \frac{[1-F(t_c;\boldsymbol{\theta}_0)]^{1/2}}{\sqrt{p_0(1-p_0)}}\sqrt{v_0}Z_1 = \sqrt{v_1}Z_1$$

by Slutsky's theorem with Lemma 2 Part 1. Along with $\mathrm{I}(M_n) \xrightarrow{p} 1$, $\widehat{p}_n \xrightarrow{p} p_0$ and the continuity of $\Phi_{\text{nor}}(\cdot)$, the continuous mapping theorem then yields

$$\Pr\left[M_n, \frac{Y_n - (n-r_n)\widehat{p}_n}{\sqrt{(n-r_n)\widehat{p}_n(1-\widehat{p}_n)}} \le z \middle| \boldsymbol{D}_n\right] \xrightarrow{d} \Phi_{\text{nor}}(z + \sqrt{v_1}Z_1).$$

Because this conditional probability is bounded by 1 and hence uniformly integrable, its convergence in distribution also implies convergence of its expectation: as $n \to \infty$,

$$\tau_n = \Pr\left[M_n, \frac{Y_n - (n-r_n)\widehat{p}_n}{\sqrt{(n-r_n)\widehat{p}_n(1-\widehat{p}_n)}} \leq z\right] = \mathrm{E}\left\{\Pr\left[M_n, \frac{Y_n - (n-r_n)\widehat{p}_n}{\sqrt{(n-r_n)\widehat{p}_n(1-\widehat{p}_n)}} \leq z \middle| \boldsymbol{D}_n\right]\right\}$$
$$\to \mathrm{E}[\Phi_{\mathrm{nor}}(z + \sqrt{v_1}Z_1)].$$

Consequently, by the above with (C.1), we have that

$$\Pr\left[\frac{Y_n - (n-r_n)\widehat{p}_n}{\sqrt{(n-r_n)\widehat{p}_n(1-\widehat{p}_n)}} \leq z\right] \to \mathrm{E}[\Phi_{\mathrm{nor}}(z + \sqrt{v_1}Z_1)] = \Pr(Z_0 + \sqrt{v_1}Z_1 \leq z),$$

where $\mathrm{E}[\Phi_{\mathrm{nor}}(z + \sqrt{v_1}Z_1)] = \Pr(Z_0 + \sqrt{v}Z_1 \leq z)$ follows for iid standard normal variables $Z_0, Z_1$. Because $z \in \mathbb{R}$ is arbitrary, we have that the cdf of the predictive root $[Y_n - (n - r_n)\widehat{p}_n]/\sqrt{(n-r_n)\widehat{p}_n(1-\widehat{p}_n)}$ converges to the cdf of $Z_0 + \sqrt{v_1}Z_1$ for any $z$ and hence $Y_n - (n-r_n)\widehat{p}_n/\sqrt{(n-r_n)\widehat{p}_n(1-\widehat{p}_n)} \xrightarrow{d} Z_0 + \sqrt{v_1}Z_1$.

The proof of Lemma 3 Part 2 closely follows the argument for Lemma 2 Part 2. Let $\{n_j\} \subset \{n\}$ be an arbitrary subsequence of indices. Because $\widehat{p}_n \xrightarrow{p} p_0 > 0$ holds by Lemma 2 along with the facts that $(n-r_n)/n \xrightarrow{p} 1 - F(t_c; \boldsymbol{\theta}_0)$ by the weak law of large numbers, while the bootstrap distribution of $\sqrt{n_k}(\widehat{p}^*_{n_k} - \widehat{p}_{n_k})$ converges in probability under Lemma 2, we may extract a further subsequence $\{n_k\} \subset \{n_j\}$ along which $\widehat{p}_{n_k} \to p_0$, $(n_k - r_{n_k})/n_k \to 1 - F(t_c; \boldsymbol{\theta}_0) > 0$ and $\sqrt{n_k}(\widehat{p}^*_{n_k} - \widehat{p}_{n_k}) \xrightarrow{d^*} \sqrt{v_0}Z_1$ converge almost surely. As in the proof of Lemma 2, we again consider the subsequence $\{n_k\}$ as $n_k \to \infty$ for a fixed point $\omega \in A$ defined by an event $A$ with $\Pr(A) = 1$ where the above-mentioned almost sure convergence holds. Fix $z \in \mathbb{R}$. Then for large $n_k$, where $n_k > r_{n_k}$ is then guaranteed, the conditional bootstrap distribution $Y^*_{n_k}|\widehat{p}^*_{n_k}$ is $\mathrm{Binomial}(n_k - r_{n_k}, \widehat{p}^*_{n_k})$ so that, by the Berry-Esseen theorem applied to the sum of $n_k - r_{n_k}$

iid $\text{Bernoulli}(\widehat{p}^*_{n_k})$ variables, we have

$$\begin{aligned}
&\Pr_*\left[\frac{Y^*_{n_k}-(n_k-r_{n_k})\widehat{p}_{n_k}}{\sqrt{(n_k-r_{n_k})\widehat{p}_{n_k}(1-\widehat{p}_{n_k})}}\leq z\Big|\widehat{p}^*_{n_k}\right]\\
=\ &\Pr_*\left[\frac{Y^*_{n_k}-(n_k-r_{n_k})\widehat{p}^*_{n_k}}{\sqrt{(n_k-r_{n_k})\widehat{p}^*_{n_k}(1-\widehat{p}^*_{n_k})}}\leq z\frac{\sqrt{\widehat{p}_{n_k}(1-\widehat{p}_{n_k})}}{\sqrt{\widehat{p}^*_{n_k}(1-\widehat{p}^*_{n_k})}}+\frac{\sqrt{n_k-r_{n_k}}(\widehat{p}_{n_k}-\widehat{p}^*_{n_k})}{\sqrt{\widehat{p}^*_{n_k}(1-\widehat{p}^*_{n_k})}}\Big|\widehat{p}^*_{n_k}\right]\\
=\ &\Phi_{\text{nor}}\left[z\frac{\sqrt{\widehat{p}_{n_k}(1-\widehat{p}_{n_k})}}{\sqrt{\widehat{p}^*_{n_k}(1-\widehat{p}^*_{n_k})}}+\frac{\sqrt{n_k-r_{n_k}}(\widehat{p}_{n_k}-\widehat{p}^*_{n_k})}{\sqrt{\widehat{p}^*_{n_k}(1-\widehat{p}^*_{n_k})}}\right]+R^*_{n_k}
\end{aligned}$$

where $\Phi_{\text{nor}}(\cdot)$ denotes the standard normal cdf and $R^*_{n_k}$ is a remainder bounded by

$$|R^*_{n_k}|\leq\frac{1}{\sqrt{n_k-r_{n_k}}}\frac{1}{\sqrt{\widehat{p}^*_{n_k}(1-\widehat{p}^*_{n_k})}}.$$

Note that we are technically assuming that $0<\widehat{p}^*_{n_k}<1$ in the conditioning of the bootstrap conditional probability above to simplify the argument, which is asymptotically valid though as $\Pr_*(0<\widehat{p}^*_{n_k}<1)\to 1$ (cf. the next line). Because $(n_k-r_{n_r})/n_k\to 1-F_0(t_c)$, $\widehat{p}_{n_k}\to p_0\in(0,1)$ and $-\sqrt{n_k}(\widehat{p}^*_{n_k}-\widehat{p}_{n_k})\stackrel{d*}{\to}\sqrt{v_0}Z_1$ (with the latter two properties also implying that $\widehat{p}^*_{n_k}\stackrel{p*}{\to}p_0$) as $n_k\to\infty$, it follows by Slutsky's theorem that $R^*_{n_k}\stackrel{p*}{\to}0$ and

$$z\frac{\sqrt{\widehat{p}_{n_k}(1-\widehat{p}_{n_k})}}{\sqrt{\widehat{p}^*_{n_k}(1-\widehat{p}^*_{n_k})}}+\frac{\sqrt{n_k-r_{n_k}}(\widehat{p}_{n_k}-\widehat{p}^*_{n_k})}{\sqrt{\widehat{p}^*_{n_k}(1-\widehat{p}^*_{n_k})}}\stackrel{d*}{\to}z+\frac{[1-F_0(t_c)]^{1/2}}{\sqrt{p_0(1-p_0)}}\sqrt{v_0}Z_1=z+\sqrt{v_1}Z_1,$$

so that the continuous mapping theorem gives

$$\Pr_*\left[\frac{Y^*_{n_k}-(n_k-r_{n_k})\widehat{p}_{n_k}}{\sqrt{(n_k-r_{n_k})\widehat{p}_{n_k}(1-\widehat{p}_{n_k})}}\leq z\Big|\widehat{p}^*_{n_k}\right]\stackrel{d*}{\to}\Phi_{\text{nor}}(z+\sqrt{v_1}Z_1)$$

by the continuity of $\Phi_{\text{nor}}(\cdot)$. Because the above bootstrap conditional probability $\Pr_*(\cdot|\widehat{p}^*_{n_k})$ is bounded by 1 and converges in distribution (under bootstrap probability $\Pr_*$ as $n_k\to\infty$), its bootstrap expectation $\text{E}_*$ (i.e., under $\Pr_*$) also converges

$$\begin{aligned}
\Pr_*\left[\frac{Y^*_{n_k}-(n_k-r_{n_k})\widehat{p}_{n_k}}{\sqrt{(n_k-r_{n_k})\widehat{p}_{n_k}(1-\widehat{p}_{n_k})}}\leq z\right]\ &=\ \text{E}_*\left\{\Pr_*\left[\frac{Y^*_{n_k}-(n_k-r_{n_k})\widehat{p}_{n_k}}{\sqrt{(n_k-r_{n_k})\widehat{p}_{n_k}(1-\widehat{p}_{n_k})}}\leq z\Big|\widehat{p}^*_{n_k}\right]\right\}\\
&\to\ \text{E}\Phi_{\text{nor}}(z+\sqrt{v_1}Z_1)=\Pr(Z_0+\sqrt{v_1}Z_1\leq z)
\end{aligned}$$

as $n_k \to \infty$. Because $z \in \mathbb{R}$ was arbitrary and the cdf of $Z_0 + \sqrt{v_1} Z_1$ is continuous, we have

$$\sup_{z\in\mathbb{R}} \left| \Pr_* \left[ \frac{Y^*_{n_k} - (n_k - r_k)\widehat{p}_{n_k}}{\sqrt{(n_k - r_k)\widehat{p}_{n_k}(1 - \widehat{p}_{n_k})}} \le z \right] - \Pr\left(Z_0 + \sqrt{v_1} Z_1 \le z\right) \right| \to 0$$

(pointwise/almost surely) as $n_k \to \infty$. As this last convergence to zero holds almost surely along the subsequence $\{n_k\} \subset \{n_j\}$ and, as the subsequence $\{n_j\}$ was arbitrary, we have shown that this convergence to zero must hold in probability (along $n$) and Lemma 3 Part 2 follows. Finally, the proof of Lemma 3 Part 3 follows by substituting $(Y^{**}_n, \widehat{p}^{**}_n)$ for $(Y^*_n, \widehat{p}^*_n)$ in the proof of Lemma 3 Part 2. □

**Proof of Theorem 1**

*Proof.* We define $\Delta_n(y) = \text{pbinom}(y, n - r_n, \widehat{p}_n) - \text{pbinom}(y, n - r_n, p_0)$. To prove Theorem 1 Part 1, without loss of generality, we often assume that $0 < \widehat{p}_n < 1$ and $r_n < n$, as $\widehat{p}_n \xrightarrow{p} p_0 \in (0, 1)$ by Lemma 2 and $\Pr(r_n = n) = [F(t_c; \boldsymbol{\theta}_0)]^n \to 0$ by $F(t_c; \boldsymbol{\theta}_0) \in (0, 1)$. Using the Berry-Esseen theorem we have,

$$\begin{aligned}\sup_{y\in\mathbb{R}} |\Delta_n(y)| &= \sup_{y\in\mathbb{R}} \left| \Phi_{\text{nor}} \left[ \frac{y - (n - r_n)p_0}{\sqrt{(n - r_n)p_0(1 - p_0)}} \right] - \Phi_{\text{nor}} \left[ \frac{y - (n - r_n)\widehat{p}_n}{\sqrt{(n - r_n)\widehat{p}_n(1 - \widehat{p}_n)}} \right] \right| + R_n \\ &= \sup_{z\in\mathbb{R}} |\Phi_{\text{nor}}(z) - \Phi_{\text{nor}}(zA_n + B_n)| + R_n,\end{aligned}$$

where $A_n \equiv \sqrt{p_0(1 - p_0)}/\sqrt{\widehat{p}_n(1 - \widehat{p}_n)}$, $B_n \equiv -(n - r_n)(\widehat{p}_n - p_0)/\sqrt{\widehat{p}_n(1 - \widehat{p}_n)}$ and $|R_n| \le 2\text{I}(\widehat{p}_n \in \{0, 1\}) + 2\text{I}(r_n = n) + [p_0(1 - p_0)]^{-1/2}(n - r_n)^{-1/2}\text{I}(r_n < n) + [\widehat{p}_n(1 - \widehat{p}_n))]^{-1/2}(n - r_n)^{-1/2}\text{I}(0 < \widehat{p}_n < 1, r_n < n)$ for $\text{I}(\cdot)$ denoting an indicator function and $\Phi_{\text{nor}}(\cdot)$ denoting the standard normal cdf. Because $\widehat{p}_n \xrightarrow{p} p_0 \in (0, 1)$ by Lemma 2 and $(n - r_n)/n \xrightarrow{p} 1 - F(t_c; \boldsymbol{\theta}_0) \in (0, 1)$ by the weak law of large numbers, we have $|R_n| \xrightarrow{p} 0$.

Note $m(a, b) \equiv \sup_{z\in\mathbb{R}} |\Phi_{\text{nor}}(z) - \Phi_{\text{nor}}(az + b)|$ is continuous as a function of $(a, b) \in (0, \infty) \times \mathbb{R}$. By Lemma 1, $(A_n, B_n) \xrightarrow{d} (1, \sqrt{v_1} Z_1)$ for $Z_1 \sim N(0, 1)$. By the continuous mapping theorem and Slutsky's theorem, we then have

$$\sup_{y\in\mathbb{R}} |\Delta_n(y)| \xrightarrow{d} m(1, \sqrt{v_1} Z_1) = \sup_{z\in\mathbb{R}} |\Phi_{\text{nor}}(z) - \Phi_{\text{nor}}(z + \sqrt{v_1} Z_1)| = 1 - 2\Phi_{\text{nor}} \left( -\frac{\sqrt{v_1}}{2} |Z_1| \right);$$

the latter supremum is determined at an argument value of $z = \mathrm{sign}(-Z_1)\sqrt{v_1}|Z_1|/2$.

For Theorem 1 Part 2, we first show that the plug-in method produces an upper prediction bound $\tilde{Y}^{PL}_{n,1-\alpha}$ such that

$$\frac{\tilde{Y}^{PL}_{n,1-\alpha} - (n-r)\widehat{p}_n}{\sqrt{(n-r)\widehat{p}_n(1-\widehat{p}_n)}} \xrightarrow{p} \Phi^{-1}_{\mathrm{nor}}(1-\alpha), \tag{C.2}$$

where $\Phi^{-1}_{\mathrm{nor}}(1-\alpha)$ denotes the $100(1-\alpha)\%$ quantile of a standard normal variable $Z_0$ with cdf $\Phi_{\mathrm{nor}}(\cdot)$, and we write $r \equiv r_n$. This follows because the plug-in method uses the $1-\alpha$ quantile of a Binomial$(n-r, \widehat{p}_n)$ random variable $Y_{0,n}$ for calibration so that $\tilde{Y}^{PL}_{n,1-\alpha} \approx \Phi^{-1}_{\mathrm{nor}}(1-\alpha)\sqrt{(n-r)\widehat{p}_n(1-\widehat{p}_n)} + (n-r)\widehat{p}_n$. More formally, by the Central Limit Theorem (or, by the Berry-Esseen theorem) applied to the sum of $(n-r)$ iid Bernoulli($\widehat{p}_n$) variables, we find

$$\sup_{z\in\mathbb{R}} \left| \Pr_* (Y_{0,n} \le z) - \Phi_{\mathrm{nor}}\left[ z\sqrt{(n-r)\widehat{p}_n(1-\widehat{p}_n)} + (n-r)\widehat{p}_n \right] \right| \le$$

$$2\mathrm{I}(\widehat{p}_n \in \{0,1\}) + 2\mathrm{I}(r=n) + \frac{1}{\sqrt{\widehat{p}_n(1-\widehat{p}_n)}}\frac{1}{\sqrt{n-r}}\mathrm{I}(0<\widehat{p}_n<1, r<n) \xrightarrow{p} 0$$

by $(n-r)/n \xrightarrow{p} 1 - F(t_c;\boldsymbol{\theta}_0) > 0$ and $\widehat{p}_n \xrightarrow{p} p_0$ again. This implies (C.2) as $\tilde{Y}^{PL}_{n,1-\alpha} = \inf\{z \in \mathbb{R} : \Pr_*(Y_{0,n} \le z) \ge 1-\alpha\}$.

By (C.2) and Lemma 3, we then have

$$\frac{Y_n - (n-r_n)\widehat{p}_n}{\sqrt{(n-r_n)\widehat{p}_n(1-\widehat{p}_n)}} - \frac{\tilde{Y}^{PL}_{n,1-\alpha} - (n-r_n)\widehat{p}_n}{\sqrt{(n-r_n)\widehat{p}_n(1-\widehat{p}_n)}} \xrightarrow{d} Z_0 + \sqrt{v_1}Z_1 - \Phi^{-1}_{\mathrm{nor}}(1-\alpha)$$

by Slutsky's theorem. By the last line, it follows immediately that

$$\begin{aligned}\Pr(Y_n \le \tilde{Y}^{PL}_{n,1-\alpha}) &= \Pr\left[\frac{Y_n - (n-r_n)\widehat{p}_n}{\sqrt{(n-r_n)\widehat{p}_n(1-\widehat{p}_n)}} \le \frac{\tilde{Y}^{PL}_{n,1-\alpha} - (n-r_n)\widehat{p}_n}{\sqrt{(n-r_n)\widehat{p}_n(1-\widehat{p}_n)}}\right] \\ &= \Pr\left[Z_0 + \sqrt{v_1}Z_1 \le \Phi^{-1}_{\mathrm{nor}}(1-\alpha)\right] \quad \text{as} \quad n\to\infty.\end{aligned}$$

Note that $v_1$ here is based on its occurrence in Lemma 3 and that, as $Z_0$ and $Z_1$ are i.i.d. standard normal, we may write

$$\begin{aligned}\Pr\left[Z_0 + \sqrt{v_1}Z_1 \le \Phi^{-1}_{\mathrm{nor}}(1-\alpha)\right] &= \mathrm{E}\Phi_{\mathrm{nor}}[\Phi^{-1}_{\mathrm{nor}}(1-\alpha) - \sqrt{v_1}Z_1] \\ &= \int_{-\infty}^{\infty} \Phi_{\mathrm{nor}}[\Phi^{-1}_{\mathrm{nor}}(1-\alpha) + \sqrt{v_1}z]\frac{1}{\sqrt{2\pi}}e^{-z^2/2}dz \equiv \Lambda_{1-\alpha}(v_1).\end{aligned}$$

Note that the probability above is 0.5 when $\alpha = 0.5$.

As a function of $v_1 > 0$ (with fixed $\alpha \in (0,1) \setminus \{0.5\}$), $\Lambda_{1-\alpha}(v_1)$ is differentiable with derivative

$$\begin{aligned}\Lambda'_{1-\alpha}(v_1) &= 0.5v_1^{-3/2}\int_{-\infty}^{\infty}\phi_{\mathrm{nor}}[\Phi^{-1}_{\mathrm{nor}}(1-\alpha)+\sqrt{v_1}z]z\frac{1}{\sqrt{2\pi}}e^{-z^2/2}dz \\ &\equiv 0.5v_1^{-3/2}\int_{0}^{\infty}[t_\alpha(z;v_1)-t_\alpha(-z;v_1)]z\frac{1}{\sqrt{2\pi}}e^{-z^2/2}dz,\end{aligned}$$

for

$$t_\alpha(z;v_1) \equiv \phi_{\mathrm{nor}}[\Phi^{-1}_{\mathrm{nor}}(1-\alpha)+\sqrt{v_1}z], \quad z \in \mathbb{R}.$$

For fixed $z > 0$ and $v_1 > 0$, it holds that $t_\alpha(z;v_1)/t_\alpha(-z;v_1) < 1$ if $\alpha \in (0, 0.5)$ (which may be checked with simple algebra), and that $t_\alpha(z;v_1)/t_\alpha(-z;v_1) > 1$ if $\alpha \in (0.5,1)$. Consequently, it follows that the derivative $\Lambda'_{1-\alpha}(v_1) < 0$ for all $v_1 > 0$ if $\alpha \in (0, 0.5)$, while $\Lambda'_{1-\alpha}(v_1) > 0$ for all $v_1 > 0$ if $\alpha \in (0.5,1)$; that is, $\Lambda_{1-\alpha}(v_1)$ is decreasing on $v_1 \in (0,\infty)$ if $\alpha \in (0, 0.5)$, and increasing on $v_1 \in (0,\infty)$ if $\alpha \in (0.5,1)$. Further, as $\Phi_{\mathrm{nor}}(\Phi^{-1}_{\mathrm{nor}}(1-\alpha)+\sqrt{v_1}z)$ is bounded by 1 and converges, for each fixed real $z \neq 0$, to the indicator function $\mathrm{I}(z > 0)$ as $v \to \infty$, the dominated convergence theorem gives

$$\lim_{v_1\to\infty}\Lambda_{1-\alpha}(v_1) = \int_0^\infty \frac{1}{\sqrt{2\pi}}e^{-z^2/2}dz = 0.5.$$

Note as well that when $\alpha \in (0, 0.5)$, we have for any $v_1 > 0$ that

$$\Lambda_{1-\alpha}(v_1) < \lim_{v_1\downarrow 0}\Lambda_{1-\alpha}(v_1) = \Lambda_{1-\alpha}(0) = 1-\alpha,$$

as $\Lambda_{1-\alpha}(v_1)$ is decreasing; when $\alpha \in (0, 0.5)$, we have instead that $\Lambda_{1-\alpha}(v_1) > 1-\alpha$ when $\alpha \in (0.5, 1)$. □

**Proof of Theorem 2**

*Proof.* For $\Psi^*_n \equiv [Y^*_n - (n-r^*_n)\widehat{p}^*_n]/\sqrt{(n-r^*_n)\widehat{p}^*_n(1-\widehat{p}^*_n)}$, we first want to show that

$$\sup_{y\in\mathbb{R}}|\mathrm{Pr}_*(\Psi^*_n \leq y) - \mathrm{Pr}(Z_0+\sqrt{v_1}Z_1 \leq y)| \xrightarrow{p} 0, \text{as } n\to\infty,$$

where $Y_n^* \sim \text{Binomial}(n - r_n^*, \widehat{p}_n)$ conditional on $(n - r_n^*)$, where $r_n^*$ is the number of events in the bootstrap sample and $\widehat{p}_n^*$ is the bootstrap version of $\widehat{p}_n$. In the bootstrap world, we have $(n - r_n^*)/n = 1 - \sum_{i=1}^n \mathrm{I}(T_i^* \leq t_c)/n$, where under bootstrap expectation

$$\mathrm{E}_* \left( \frac{n - r_n^*}{n} \right) = 1 - \Pr_*(T_1^* \leq t_c) \xrightarrow{p} 1 - F(t_c, \boldsymbol{\theta}_0) > 0,$$

by the assumption that $\Pr_*(T_1^* \leq t_c)$ is consistent for $F(t_c; \boldsymbol{\theta}_0)$ (e.g., $\Pr_*(T_1^* \leq t_c) = F(t_c; \widehat{\boldsymbol{\theta}}_n)$), and likewise

$$\begin{aligned} \mathrm{Var}_* \left( \frac{n - r_n^*}{n} \right) &= \mathrm{Var}_* \left[ \frac{1}{n} \sum_{i=1}^n \mathrm{I}(T_i^* \leq t_c) \right] \\ &= \frac{1}{n} \Pr_* \left( T_1^* \leq t_c \right) \Pr_* \left( T_1^* > t_c \right) \leq \frac{1}{n} \xrightarrow{p} 0, \text{ as } n \to \infty. \end{aligned}$$

Hence, the convergence of these two bootstrap moments implies that $(n - r_n^*)/n$ converges in bootstrap probability or $(n - r_n^*)/ \xrightarrow{p*} 1 - F(t_c; \boldsymbol{\theta}_0)$ (in probability); that is, for any subsequence $\{n_j\} \subset \{n\}$, there exists a further subsequence $\{n_k\} \subset \{n_j\}$ where with probability 1,

$$\Pr_* \left[ \left| \frac{n_k - r_{n_k}^*}{n_k} - 1 + F(t_c; \boldsymbol{\theta}_0) \right| > \epsilon \right] \to 0$$

holds as $n_k \to \infty$ for each given $\epsilon > 0$. Choose a subsequence $\{n_k\}$ where together $(n_k - r_{n_k}^*)/n_k \xrightarrow{p^*} 1 - F(t_c; \boldsymbol{\theta}_0) \in (0, 1)$ (by the above) and $\sqrt{n_k - r_{n_k}}(\widehat{p}_{n_k}^* - \widehat{p}_{n_k})/\sqrt{\widehat{p}_{n_k}(1 - \widehat{p}_{n_k})} \xrightarrow{d^*} \sqrt{v_1} Z_1$ (by Lemma 3) and $\widehat{p}_{n_k} \to p_0 \in (0, 1)$ and $(n_k - r_{n_k})/n_k \to 1 - F(t_c; \boldsymbol{\theta}_0)$ hold as $n_k \to \infty$ with probability 1. Now conditional on $(n_k - r_{n_k}^*), \widehat{p}_{n_k}^*$ (here, without a loss of generality, assuming $n - r_{n_k}^* > 0$, $0 < \widehat{p}_{n_k}^* < 1$) and for fixed $y \in \mathbb{R}$, we can write

$$\begin{aligned} &\Pr_*(\Psi_{n_k}^* \leq y | n_k - r_{n_k}^*, \widehat{p}_{n_k}^*) \\ =&\Pr_* \left[ \frac{Y_{n_k}^* - (n_k - r_{n_k}^*)\widehat{p}_{n_k}}{\sqrt{(n_k - r_{n_k}^*)\widehat{p}_{n_k}(1 - \widehat{p}_{n_k})}} \leq y \frac{\sqrt{(n_k - r_{n_k}^*)\widehat{p}_{n_k}^*(1 - \widehat{p}_{n_k}^*)}}{\sqrt{(n_k - r_{n_k}^*)\widehat{p}_{n_k}(1 - \widehat{p}_{n_k})}} - \frac{\sqrt{n_k - r_{n_k}^*}(\widehat{p}_{n_k}^* - \widehat{p}_{n_k})}{\sqrt{\widehat{p}_{n_k}(1 - \widehat{p}_{n_k})}} \right| n_k - r_{n_k}^*, \widehat{p}_{n_k}^* \right] \\ =&\Phi_{\text{nor}} \left[ y \frac{\sqrt{(n_k - r_{n_k}^*)\widehat{p}_{n_k}^*(1 - \widehat{p}_{n_k}^*)}}{\sqrt{(n_k - r_{n_k}^*)\widehat{p}_{n_k}(1 - \widehat{p}_{n_k})}} - \frac{\sqrt{n_k - r_{n_k}^*}(\widehat{p}_{n_k}^* - \widehat{p}_{n_k})}{\sqrt{\widehat{p}_{n_k}(1 - \widehat{p}_{n_k})}} \right] + R_{n_k}^*, \end{aligned}$$

by the Berry-Esseen theorem, where the remainder $R^*_{n_k}$ is bounded by

$$\left|R^*_{n_k}\right| \leq 2\mathrm{I}(\widehat{p}^*_{n_k} \in \{0,1\}) + 2\mathrm{I}(r^*_{n_k} = n_k) + \frac{1}{\sqrt{\widehat{p}^*_{n_k}(1-\widehat{p}^*_{n_k})}} \frac{1}{\sqrt{n_k - r_{n_k}}} \mathrm{I}(0 < \widehat{p}^*_{n_k} < 1, r_{n_k} < n_k),$$

for some constant if $n_k - r^*_{n_k} > 0$. Then $\left|R^*_{n_k}\right| \xrightarrow{p^*} 0$ follows because $1/\sqrt{n_k - r^*_{n_k}} \xrightarrow{p^*} 0$ and $\widehat{p}^*_{n_k} \xrightarrow{p*} p_0 \in (0,1)$ as $n_k \to \infty$. It also holds that

$$\frac{\sqrt{n_k - r^*_{n_k}}}{\sqrt{n_k - r_{n_k}}} \frac{\sqrt{n_k - r_{n_k}}(\widehat{p}^*_{n_k} - \widehat{p}_{n_k})}{\sqrt{\widehat{p}_{n_k}(1-\widehat{p}_{n_k})}} \xrightarrow{d^*} \sqrt{v_1} Z_1,$$

as $n_k \to \infty$ by Slutsky's theorem so that, by the continuous mapping theorem, we have

$$\Pr_*\left(\Psi^*_{n_k} \leq y | n_k - r^*_{n_k}, \widehat{p}^*_{n_k}\right) \xrightarrow{d^*} \Phi_{\mathrm{nor}}\left(y + \sqrt{v_1} Z_1\right).$$

Because the conditional probability is bounded by 1, we have that expectations converge in the bootstrap world as

$$\Pr_*(\Psi^*_{n_k} \leq y) = \mathrm{E}_*\left[\Pr_*\left(\Psi^*_{n_k} \leq y | n_k - r^*_{n_k}, \widehat{p}^*_{n_k}\right)\right] \to \mathrm{E}\Phi_{\mathrm{nor}}(y + \sqrt{v_1} Z_1) = \Pr(Z_0 + \sqrt{v_1} Z_1 \leq y)$$

as $n_k \to \infty$. Because the real $y \in \mathbb{R}$ was arbitrary, we have $\Psi^*_{n_k} \xrightarrow{d^*} Z_0 + \sqrt{v_1} Z_1$ as $n_k \to \infty$ (holding with probability 1 along $n_k$) or

$$\sup_{y \in \mathbb{R}} \left|\Pr_*(\Psi^*_{n_k} \leq y) - \Pr(Z_0 + \sqrt{v_1} Z_1 \leq y)\right| \to 0, \tag{C.3}$$

as $n_k \to \infty$ (with probability 1).

Next we prove that $U^*_n = \mathrm{pbinom}\left(Y^*_n, n - r^*_n, \widehat{p}^*_n\right) \xrightarrow{d^*} \Phi_{\mathrm{nor}}\left(Z_0 + \sqrt{v_1} Z_1\right)$ (in probability). For $U^*_n$ and $u \in (0,1)$, we write

$$\begin{aligned}\Pr_*\left(U^*_n \leq u\right) &= \Pr_*\left[Y^*_n \leq \mathrm{qbinom}(u, n - r^*_n, \widehat{p}^*_n)\right] \\ &= \Pr_*\left[\Psi^*_n \leq \Phi^{-1}_{\mathrm{nor}}(u) + \frac{L^*_n}{\sqrt{(n - r^*_n)\widehat{p}^*_n(1-\widehat{p}^*_n)}}\right],\end{aligned}$$

where $L_n^* = \text{qbinom}(u, n-r_n^*, \widehat{p}_n^*) - \Phi_{\text{nor}}^{-1}(u)\sqrt{(n-r_n^*)\widehat{p}_n^*(1-\widehat{p}_n^*)} - (n-r_n^*)\widehat{p}_n^*$. By the Berry-Esseen theorem and $n - r_{n_k}^* \xrightarrow{p^*} \infty$, $\widehat{p}_{n_k}^* \xrightarrow{p^*} p$ along the subsequence $n_k$ (with probability 1), we have

$$\frac{L_{n_k}^*}{\sqrt{(n_k - r_{n_k}^*)\widehat{p}_{n_k}^*(1-\widehat{p}_{n_k}^*)}} = \frac{\text{qbinom}(u, n_k - r_{n_k}^*, \widehat{p}_n^*) - (n_k - r_{n_k}^*)\widehat{p}_{n_k}}{\sqrt{(n_k - r_{n_k}^*)\widehat{p}_{n_k}^*(1-\widehat{p}_{n_k}^*)}} - \Phi_{\text{nor}}^{-1}(u)$$
$$\xrightarrow{p^*} \Phi_{\text{nor}}^{-1}(u) - \Phi_{\text{nor}}^{-1}(u) = 0.$$

By this and (C.3), it follows that

$$\Pr_*\left(U_{n_k}^* \le u\right) \to \Pr\left[Z_0 + \sqrt{v_1}Z_1 \le \Phi_{\text{nor}}^{-1}(u)\right] = \Pr\left[\Phi_{\text{nor}}(Z_0 + \sqrt{v_1}Z_1) \le u\right]$$

as $n_k \to \infty$ for each $u \in (0,1)$ (with probability 1). Because the subsequence $\{n_j\}$ was arbitrary, we have $U_n^* \xrightarrow{d^*} \Phi_{\text{nor}}(Z_0 + \sqrt{v_1}Z_1)$ in probability as $n \to \infty$ or

$$\sup_{u\in(0,1)} \left|\Pr_*(U_n^* \le u) - \Pr[\Phi_{\text{nor}}(Z_0 + \sqrt{v_1}Z_1) \le u]\right| \xrightarrow{p} 0, \tag{C.4}$$

as $n \to \infty$.

The $100(1-\alpha)\%$ upper calibration prediction bound is $\tilde{Y}_{n,1-\alpha}^C$ such that

$$\frac{\tilde{Y}_{n,1-\alpha}^C - (n-r_n)\widehat{p}_n}{\sqrt{(n-r_n)\widehat{p}_n(1-\widehat{p}_n)}} - \Phi_{\text{nor}}^{-1}(U_{1-\alpha}^*) \xrightarrow{p} 0, \tag{C.5}$$

where $U_{n,1-\alpha}^*$ is the $1-\alpha$ quantile of $U_n^*$, which follows by the Berry-Esseen theorem applied to the Binomial$(n-r_n, \widehat{p}_n)$ distribution. Let $\kappa_{1-\alpha}$ be the $1-\alpha$ quantile of $\Phi_{\text{nor}}(Z_0 + \sqrt{v_1}Z_1)$. Then $\kappa_{1-\alpha} - U_{n,1-\alpha}^* \xrightarrow{p} 0$ holds by (C.4). Thus from this and (C.5) along with the continuity of $\Phi_{\text{nor}}$ and $\Phi_{\text{nor}}^{-1}$, it follows that

$$\Phi_{\text{nor}}\left[\frac{\tilde{Y}_{n,1-\alpha}^C - (n-r_n)\widehat{p}_n}{\sqrt{(n-r_n)\widehat{p}_n(1-\widehat{p}_n)}}\right] \xrightarrow{p} \Phi_{\text{nor}}\left[\Phi_{\text{nor}}^{-1}(\kappa_{1-\alpha})\right] = \kappa_{1-\alpha}. \tag{C.6}$$

Hence, by Lemma 2, (C.6) and Slutsky's theorem, we have

$$
\begin{aligned}
&\Pr(Y_n \leq \tilde{Y}^C_{n,1-\alpha}) \\
&= \Pr\left\{\Phi_{\text{nor}}\left[\frac{Y_n - (n-r_n)\widehat{p}_n}{\sqrt{(n-r_n)\widehat{p}_n(1-\widehat{p}_n)}}\right] - \kappa_{1-\alpha} \leq \Phi_{\text{nor}}\left[\frac{\tilde{Y}^C_{n,1-\alpha} - (n-r_n)\widehat{p}_n}{\sqrt{(n-r_n)\widehat{p}_n(1-\widehat{p}_n)}}\right] - \kappa_{1-\alpha}\right\} \\
&\to \Pr\left[\Phi_{\text{nor}}(Z_0 + \sqrt{v_1}Z_1) - \kappa_{1-\alpha} \leq \kappa_{1-\alpha} - \kappa_{1-\alpha}\right] = 1-\alpha.
\end{aligned}
$$

The $1-\alpha$ lower prediction bound $\underset{\sim}{Y}^C_{n,1-\alpha}$ is equal to $\tilde{Y}^C_{n,\alpha}$ or off by 1, so immediately we have $\Pr(Y_n \geq \underset{\sim}{Y}^C_{n,1-\alpha}) = 1-\alpha$. □

**Proof of Theorem 3**

*Proof.* To prove Theorem 3 Part 1, let $q_{1-\alpha} \equiv \inf\{z \in \mathbb{R} : \Pr(Z_0 + \sqrt{v_1}Z_1 \leq z) \geq 1-\alpha\}$ denote the $1-\alpha$ quantile of the distribution of $Z_0 + \sqrt{v_1}Z_1$, where $Z_1, Z_0$ are iid standard normal variables with $v_1 > 0$ as in Lemma 3. Let $Y^*_n \sim$ Binomial$(n - r^*_n, \widehat{p}_n)$ and $\widehat{Q}_{n,1-\alpha} \equiv \inf\{z \in \mathbb{R} : G^*_n(z) \geq 1-\alpha\}$ denote $1-\alpha$ quantile of the bootstrap distribution of $[Y^*_n - (n-r)\widehat{p}_n]/\sqrt{(n-r)\widehat{p}_n(1-\widehat{p}_n)}$ with cdf $G^*_n(z) \equiv \Pr_*\{[Y^*_n - (n-r)\widehat{p}_n]/\sqrt{(n-r)\widehat{p}_n(1-\widehat{p}_n)} \leq z\}$, $z \in \mathbb{R}$. Then, it follows from Lemma 3 Part 2 that $\widehat{Q}_{n,1-\alpha} \xrightarrow{p} q_{1-\alpha}$ as $n \to \infty$. To see this, for any given $\epsilon > 0$, we have $G^*_n(q_{1-\alpha} - \epsilon) \xrightarrow{p} \Pr(Z_0 + \sqrt{v_1}Z_1 \leq q_{1-\alpha} - \epsilon) < 1-\alpha$ and $G^*_n(q_{1-\alpha} + \epsilon) \xrightarrow{p} \Pr\left(Z_0 + \sqrt{v_1}Z_1 \leq q_{1-\alpha} + \epsilon\right) > 1-\alpha$ by Lemma 3 Part 2. Hence, $\Pr\left[G^*_n(q_{1-\alpha} - \epsilon) < 1-\alpha < G^*_n(q_{1-\alpha} + \epsilon)\right] \to 1$ as $n \to \infty$, and this event implies that $q_{1-\alpha} - \epsilon \leq \widehat{Q}_{n,1-\alpha} \leq q_{1-\alpha} + \epsilon$ holds so that $\Pr(|\widehat{Q}_{n,1-\alpha} - q_{1-\alpha}| \leq \epsilon) \to 1$. By definition, the upper prediction bound for $Y_n$ is given by

$$\tilde{Y}^{DB}_{n,1-\alpha} = \widehat{Q}_{n,1-\alpha}\sqrt{(n-r)\widehat{p}_n(1-\widehat{p}_n)} + (n-r)\widehat{p}_n.$$

Then using that $[Y_n - (n-r)\widehat{p}_n]/[\sqrt{(n-r)\widehat{p}_n(1-\widehat{p}_n)}] - \widehat{Q}_{n,1-\alpha} \xrightarrow{d} Z_0 + \sqrt{v_1}Z_1 - q_{1-\alpha}$ (a normal random variable with mean $-q_{1-\alpha}$ and variance $1 + v_1$) by Slutsky's theorem from

$\widehat{Q}_{n,1-\alpha} \xrightarrow{p} q_{1-\alpha}$ along with Lemma 3 Part 1, we have that

$$
\begin{aligned}
\Pr(Y_n \leq \tilde{Y}^{DB}_{n,1-\alpha}) &= \Pr\left[\frac{Y_n - (n-r)\widehat{p}_n}{\sqrt{(n-r)\widehat{p}_n(1-\widehat{p}_n)}} \leq \widehat{Q}_{n,1-\alpha}\right] \\
&= \Pr\left[\frac{Y_n - (n-r)\widehat{p}_n}{\sqrt{(n-r)\widehat{p}_n(1-\widehat{p}_n)}} - \widehat{Q}_{n,1-\alpha} \leq 0\right] \\
&\to \Pr\left(Z_0 + \sqrt{v_1}Z_1 - q_{1-\alpha} \leq 0\right) \\
&= \Pr\left(Z_0 + \sqrt{v_1}Z_1 \leq q_{1-\alpha}\right) = 1-\alpha.
\end{aligned}
$$

This establishes Theorem 3 Part 1. Again, the lower prediction bound $\underset{\sim}{Y}^{DB}_{n,1-\alpha}$ is equal to $\tilde{Y}^{DB}_{n,\alpha}$ or $\tilde{Y}^{DB}_{n,\alpha}$-1, which implies that $\lim_{n\to\infty}\Pr(Y_n \geq \underset{\sim}{Y}^{DB}_{n,1-\alpha}) = 1 - \lim_{n\to\infty}\Pr(Y_n \leq \tilde{Y}^{DB}_{n,\alpha}) = 1-\alpha$.

The proof of Theorem 3 Part 2 follows analogously by replacing $(Y_n^*, \widehat{p}_n^*)$ with $(Y_n^{**}, \widehat{p}_n^{**})$ and applying Lemma 3 Part 3. □

# Section D Extending the Theorems to Multiple-Cohort Data

For multiple-cohort data, we assume that $\lim_{n\to\infty} n_s/n \to c_s \in [0,1]$ exists for $s = 1, ..., S$, where $\sum_{s=1}^{S} c_s = 1$, and then describe some minor modifications needed to the assumptions of Theorem 1 and 2. As in Theorem 1, based on the censored sample, an estimator of $\boldsymbol{\theta} \in \mathbb{R}^q$ is assumed to satisfy $\sqrt{n}(\widehat{\boldsymbol{\theta}}_n - \boldsymbol{\theta}_0) \xrightarrow{d} \text{MVN}(0, \boldsymbol{V}_0)$ as $n \to \infty$ , and its bootstrap counterpart approximation is assumed to be distributionally consistent as in Theorem 2. For the multiple-cohort case, the small change to Theorem 1 conditions is that, for each cohort $s$, we assume that (with respect to the censoring time $t_c^s$ of the cohort) $F(t_c^s;\boldsymbol{\theta})$ is continuous at $\boldsymbol{\theta}_0$ with $F(t_c^s;\boldsymbol{\theta}_0) \in (0,1)$, and that the conditional probability $p_s = \pi_s(\boldsymbol{\theta}) = [F(t_c^s+\Delta;\boldsymbol{\theta}) - F(t_c^s;\boldsymbol{\theta})] \,/\, [1-F(t_c^s;\boldsymbol{\theta})]$ is continuously differentiable in a neighborhood of $\boldsymbol{\theta}_0$ with gradient $\nabla_0^s = \partial\pi_s(\boldsymbol{\theta})/\partial\boldsymbol{\theta}|_{\boldsymbol{\theta}=\boldsymbol{\theta}_0}$, where $p_{0,s} = \pi_s(\boldsymbol{\theta}_0) \in (0,1)$; assume also that $\nabla_0^s$ is non-zero for some cohort $s$ with $c_s > 0$. Then, the same statement of Theorem 1 continues to

hold for the multiple-cohort setting upon redefining the term $v_1 > 0$ to be

$$\frac{1}{\sum_{s=1}^{S} c_s[1-F(t_c^s;\boldsymbol{\theta}_0)]p_{0,s}(1-p_{0,s})}\begin{pmatrix} c_1[1-F(t_c^1;\boldsymbol{\theta}_0)] \\ \vdots \\ c_S[1-F(t_c^S;\boldsymbol{\theta}_0)] \end{pmatrix}^t \Gamma_0^t V_0 \Gamma_0 \begin{pmatrix} c_1[1-F(t_c^1;\boldsymbol{\theta}_0)] \\ \vdots \\ c_S[1-F(t_c^S;\boldsymbol{\theta}_0)] \end{pmatrix}$$

where $\Gamma_0$ is now a $q \times S$ matrix given by

$$\Gamma_0 \equiv \left[\nabla_0^1 \cdots \nabla_0^S\right].$$

With this change, statements of Lemmas 1-2 also remain valid.

Statements of Theorem 2 and Theorem 3 (and Lemma 3) also continue to hold, if we naturally extend the bootstrap consistency assumption of Theorem 2 so that $\Pr_*(T_1^* \le t_c^s) \xrightarrow{p} F(t_c^s;\boldsymbol{\theta}_0)$ is assumed for any cohort with $c_s > 0$.

We next describe some (mostly minor) modifications for the proofs to hold under multiple-cohort data.

**Extending Lemma 1**

Lemma 1 does not change for multiple-cohort data.

**Extending Lemma 2**

In multiple-cohort data, the ML estimator of conditional probabilities $\widehat{\boldsymbol{p}}_n$ is a vector of length $S$, where $S$ is the number of cohorts. To extend Lemma 2 Part 1, $\sqrt{n}(\widehat{\boldsymbol{p}}_n - \boldsymbol{p}_0) \xrightarrow{d} X_0$ now holds, where $X_0 \sim \mathrm{MVN}(\mathbf{0}, \Gamma_0^t V_0 \Gamma_0)$, with $\Gamma_0$ as above, using the delta method and $\boldsymbol{p}_0 = (p_{0,1}, \ldots, p_{0,S}) \equiv [\pi_1(\boldsymbol{\theta}_0), \ldots, \pi_S(\boldsymbol{\theta}_0)]$. For Lemma 2 Part 2, it holds that

$$\sup_{x\in\mathbb{R}, \|a\|=1} \left|\Pr_*(a^T\sqrt{n}(\widehat{\boldsymbol{p}}_n^* - \boldsymbol{p}_0) \le z) - \Pr(a^T X_0 \le z)\right| \xrightarrow{p} 0.$$

The same changes are made to Lemma 2 Part 3.

**Extending Lemma 3**

The predictand can be written as $Y_n = \sum_{s=1}^{S} Y_s$, where $Y_{n_s}$ is the number of events during future time interval in cohort $s$. Here $n_s$ is the size of the cohort $s$. Thus for re-formulating

Lemma 3 Part 1, we write

$$\begin{aligned}
A_n \equiv & \frac{Y_n - \sum_{s=1}^{S}(n_s - r_{n_s})\widehat{p}_n^s}{\sqrt{\sum_{s=1}^{S}(n_s - r_{n_s})\widehat{p}_n^s(1-\widehat{p}_n^s)}} \\
= & \frac{Y_n - \sum_{s=1}^{S}(n_s - r_{n_s})p_{0,s}}{\sqrt{\sum_{s=1}^{S}(n_s - r_{n_s})p_{0,s}(1-p_{0,s})}} \frac{\sqrt{\sum_{s=1}^{S}(n_s - r_{n_s})p_{0,s}(1-p_{0,s})}}{\sqrt{\sum_{s=1}^{S}(n_s - r_{n_s})\widehat{p}_n^s(1-\widehat{p}_n^s)}} + \frac{\sum_{s=1}^{S}(n_s - r_{n_s})(p_{0,s}-\widehat{p}_n^s)}{\sqrt{\sum_{s=1}^{S}(n_s - r_{n_s})\widehat{p}_n^s(1-\widehat{p}_n^s)}} \\
\equiv & A_{1n}c_n + A_{2n}
\end{aligned}$$

as the sum of two terms, where the second term can be re-written as

$$A_{2n} \equiv \frac{\sum_{s=1}^{S}(n_s - r_{n_s})(p_{0,s}-\widehat{p}_n^s)}{\sqrt{\sum_{s=1}^{S}(n_s - r_{n_s})\widehat{p}_n^s(1-\widehat{p}_n^s)}} = \sum_{s=1}^{S} \frac{\frac{n_s - r_{n_s}}{n}}{\sqrt{\sum_{j=1}^{S}\frac{n_j - r_{n_j}}{n}\widehat{p}_n^j(1-\widehat{p}_n^j)}}\sqrt{n}(p_{0,s}-\widehat{p}_n^s).$$

For each $s = 1, \ldots, S$, note that $(n_s - r_{n_s})/n \to c_s[1-F(t_c^s;\boldsymbol{\theta}_0)]$ by the weak law of large numbers and that the normal limit of $\sqrt{n}(p_{0,s}-\widehat{p}_n^s)$ is determined by the normal limit of $\sqrt{n}(\widehat{\boldsymbol{p}}_n - \boldsymbol{p}_0)$ through $\sqrt{n}(\widehat{\boldsymbol{\theta}}_n - \boldsymbol{\theta}_0)$. Additionally, by the consistency of $\widehat{\boldsymbol{\theta}}_n$ and the smoothness of $\pi_s(\boldsymbol{\theta})$ we have that $\widehat{p}_n^s = \pi_s(\widehat{\boldsymbol{\theta}}_n) \xrightarrow{p} \pi_s(\boldsymbol{\theta}_0) = p_{0,s} \in (0,1)$ for each $s = 1, \ldots, S$. Hence, it holds that $A_{2n} \xrightarrow{d} \sqrt{v_1}Z_1$ in distribution (for $v_1$ given above and standard normal variable $Z_1$), which follows from Slutsky's theorem and the normal limit of $\sqrt{n}(\widehat{\boldsymbol{p}}_n - \boldsymbol{p}_0)$. The previous arguments also show that

$$c_n \equiv \frac{\sqrt{\sum_{s=1}^{S}(n_s - r_{n_s})p_{0,s}(1-p_{0,s})}}{\sqrt{\sum_{s=1}^{S}(n_s - r_{n_s})\widehat{p}_n^s(1-\widehat{p}_n^s)}} \xrightarrow{p} 1.$$

Finally, as in the original proof of Lemma 3, we may apply the Berry-Esseen theorem to determine a normal limit for the sum $A_{1n}$ appearing in $A_n$, as a sum of non-identical but independent Bernoulli random variables, conditional on the censored multiple-cohort data. Namely, for fixed real $z \in \mathbb{R}$, it analogously holds that $|\Pr(A_n \le z) - \mathrm{E}[\Phi_{\text{nor}}(z - A_{2n}/c_n)]| \to 0$ from the Berry-Esseen theorem, where $\mathrm{E}\Phi_{\text{nor}}(z - A_{2n}/c_n) \to \mathrm{E}[\Phi_{\text{nor}}(z - \sqrt{v_1}Z_1)] = \Pr(Z_0 + \sqrt{v_1}Z_1)$ holds for independent standard normal variables $Z_0, Z_1$ (as $\Phi_{\text{nor}}(z - A_{2n}/c_n)$ converges to $\Phi_{\text{nor}}(z - \sqrt{v_1}Z_1)$ in both distribution and expectation by the continuous mapping theorem combined with $A_{2n}/c_n \xrightarrow{d} \sqrt{v_1}Z_1$).

Lemma 3 Part 2 and Lemma 3 Part 3 remain as re-casts of Lemma 3 Part 1 in the bootstrap world.

**Extension of Theorems**

In the multiple-cohort case, the predictand has a Poisson-binomial distribution. Then the proof follows the same method as in Binomial case. We only need to replace the standardized form of predictand with the Poisson-binomial counterpart.

# Section E Simulation Results of Section 8 & the Bearing Cage Data

Section 8 provides a summary of the results from our simulation study. This section provides a graphical summary of the results at the other factor-level combinations used in the study.

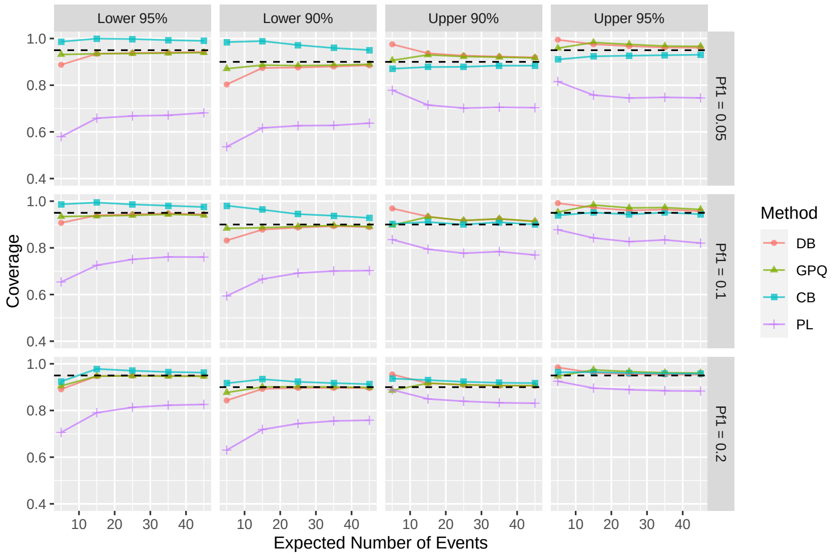


Figure 6: Coverage probabilities versus expected number of events for the direct-bootstrap, GPQ-bootstrap, calibration-bootstrap, and plug-in methods when $d = p_{f2} - p_{f1} = 0.1$ and $\beta = 0.5$.

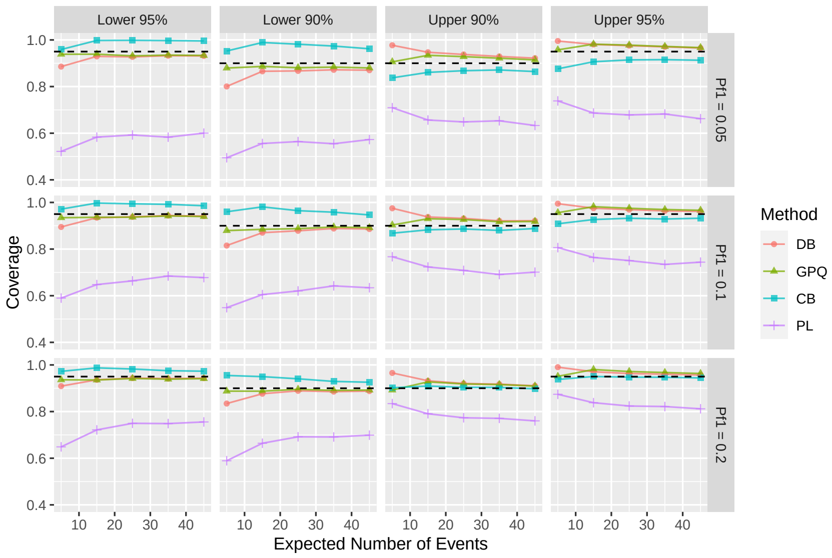


Figure 7: Coverage probabilities versus expected number of events for the direct-bootstrap, GPQ-bootstrap, calibration-bootstrap, and plug-in methods when $d = p_{f2} - p_{f1} = 0.2$ and $\beta = 0.5$.

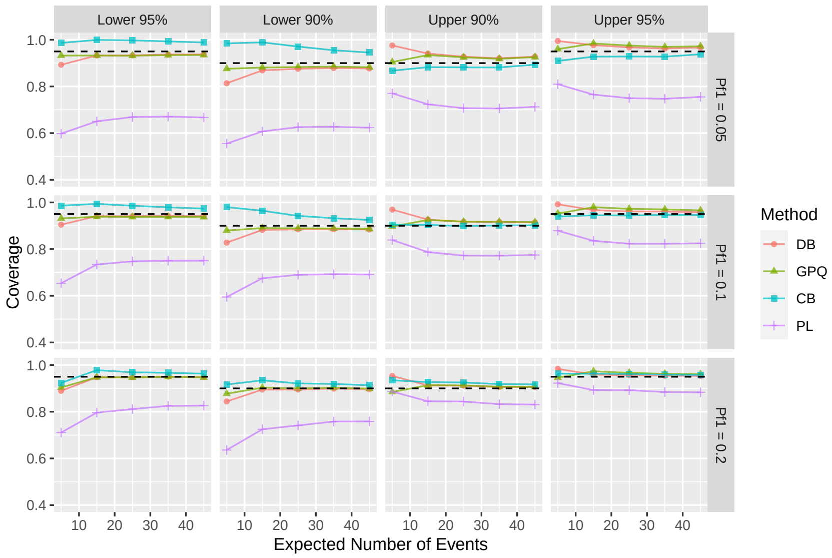


Figure 8: Coverage probabilities versus expected number of events for the direct-bootstrap, GPQ-bootstrap, calibration-bootstrap, and plug-in methods when $d = p_{f2} - p_{f1} = 0.1$ and $\beta = 0.8$.

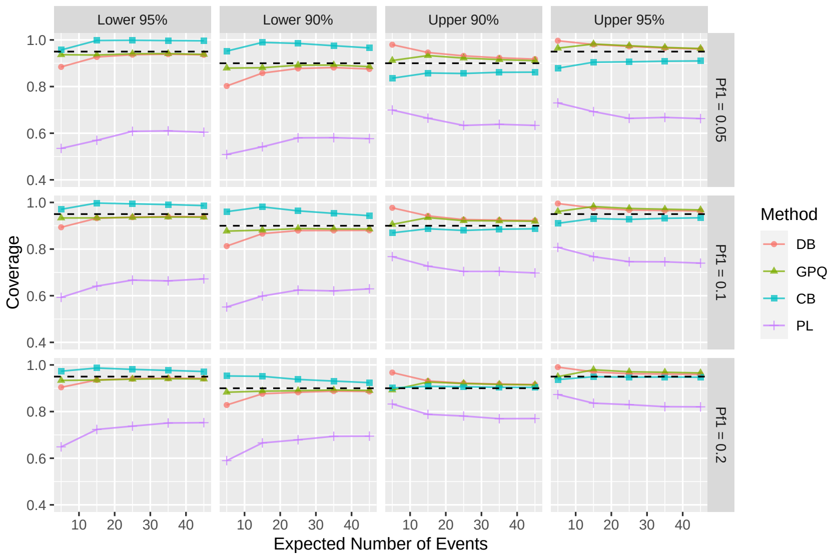


Figure 9: Coverage probabilities versus expected number of events for the direct-bootstrap, GPQ-bootstrap, calibration-bootstrap, and plug-in methods when $d = p_{f2} - p_{f1} = 0.2$ and $\beta = 0.8$.

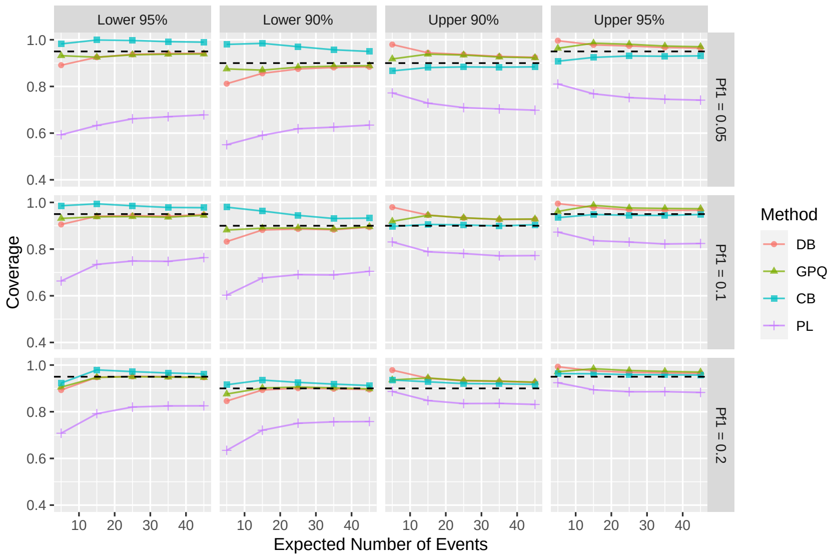


Figure 10: Coverage probabilities versus expected number of events for the direct-bootstrap, GPQ-bootstrap, calibration-bootstrap, and plug-in methods when $d = p_{f2} - p_{f1} = 0.1$ and $\beta = 2$.

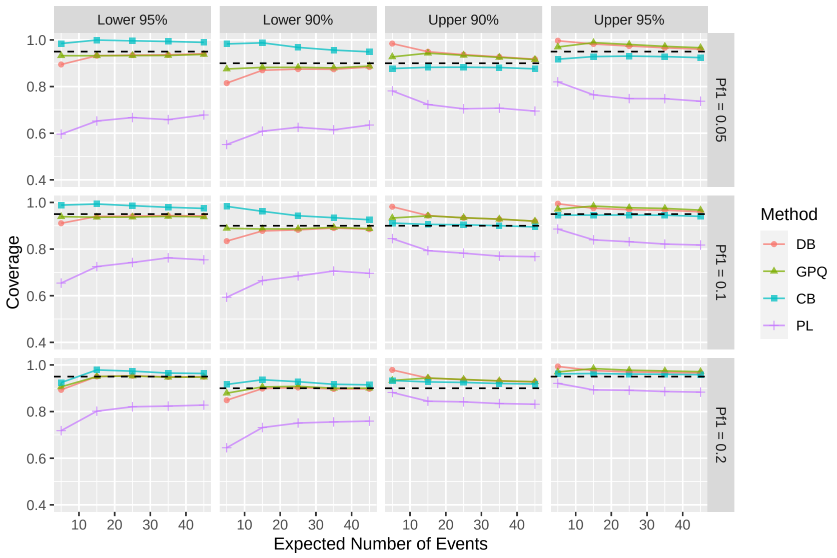


Figure 11: Coverage probabilities versus expected number of events for the direct-bootstrap, GPQ-bootstrap, calibration-bootstrap, and plug-in methods when $d = p_{f2} - p_{f1} = 0.1$ and $\beta = 4$.

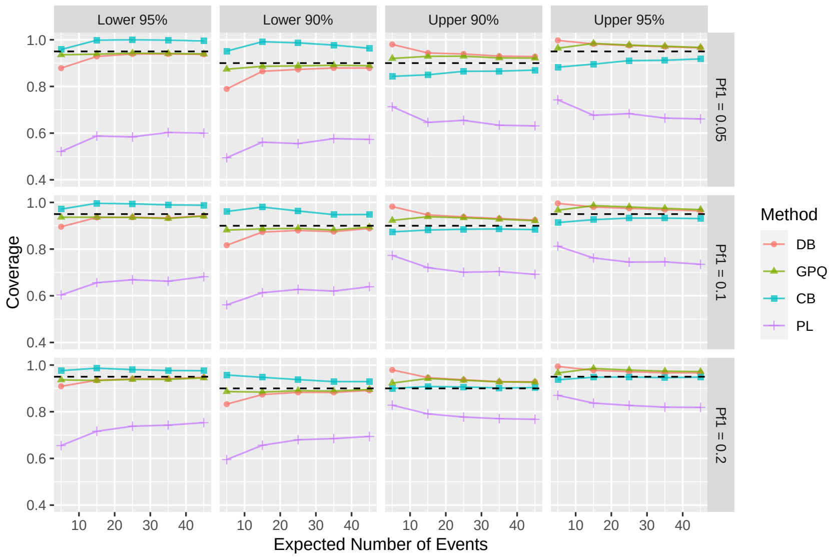


Figure 12: Coverage probabilities versus expected number of events for the direct-bootstrap, GPQ-bootstrap, calibration-bootstrap, and plug-in methods when $d = p_{f2} - p_{f1} = 0.2$ and $\beta = 4$.

Table 6 gives the data for the bearing cage example.

| Group $i$ | Hours in Service | Group Size $n_i$ | Failed $r_i$ | At Risk $n_i - r_i$ | $\hat{p}_i$ | $(n_i - r_i) \times \hat{p}_i$ |
|---|---|---|---|---|---|---|
| 1 | 50 | 288 | 0 | 288 | 0.000763 | 0.2196 |
| 2 | 150 | 148 | 0 | 148 | 0.001158 | 0.1714 |
| 3 | 250 | 125 | 1 | 124 | 0.001558 | 0.1932 |
| 4 | 350 | 112 | 1 | 111 | 0.001962 | 0.2178 |
| 5 | 450 | 107 | 1 | 106 | 0.002369 | 0.2511 |
| 6 | 550 | 99 | 0 | 99 | 0.002778 | 0.2750 |
| 7 | 650 | 110 | 0 | 110 | 0.003189 | 0.3508 |
| 8 | 750 | 114 | 0 | 114 | 0.003602 | 0.4106 |
| 9 | 850 | 119 | 0 | 119 | 0.004016 | 0.4779 |
| 10 | 950 | 128 | 0 | 128 | 0.004432 | 0.5673 |
| 11 | 1050 | 124 | 2 | 122 | 0.004848 | 0.5915 |
| 12 | 1150 | 93 | 0 | 93 | 0.005266 | 0.4898 |
| 13 | 1250 | 47 | 0 | 47 | 0.005685 | 0.2672 |
| 14 | 1350 | 41 | 0 | 41 | 0.006105 | 0.2503 |
| 15 | 1450 | 27 | 0 | 27 | 0.006525 | 0.1762 |
| 16 | 1550 | 12 | 1 | 11 | 0.006946 | 0.0764 |
| 17 | 1650 | 6 | 0 | 6 | 0.007368 | 0.0442 |
| 18 | 1750 | 0 | 0 | 0 | 0.007791 | 0 |
| 19 | 1850 | 1 | 0 | 1 | 0.008214 | 0.0082 |
| 20 | 1950 | 0 | 0 | 0 | 0.008638 | 0 |
| 21 | 2050 | 2 | 0 | 2 | 0.009062 | 0.0181 |
| Total | 1703 | | 6 | | | 5.062 |

Table 6: Bearing cage data: future-failure risk analysis for the next year (300 hours of service per unit).

# Section F Additional Distributional Comparisons

Section 10 of the main manuscript compares the Weibull, lognormal, and Fréchet distributions (as examples of event or failure time models) and presents the plots for $\beta = 2$. Additional plots for $\beta = 1, 4$ are given here. The intent of these plots is to show how different models may vary in their probabilities of future failure events, while having similar percentiles in an initial range where data are observed (e.g., prior to a censoring time $t_c$ for single-cohort data).

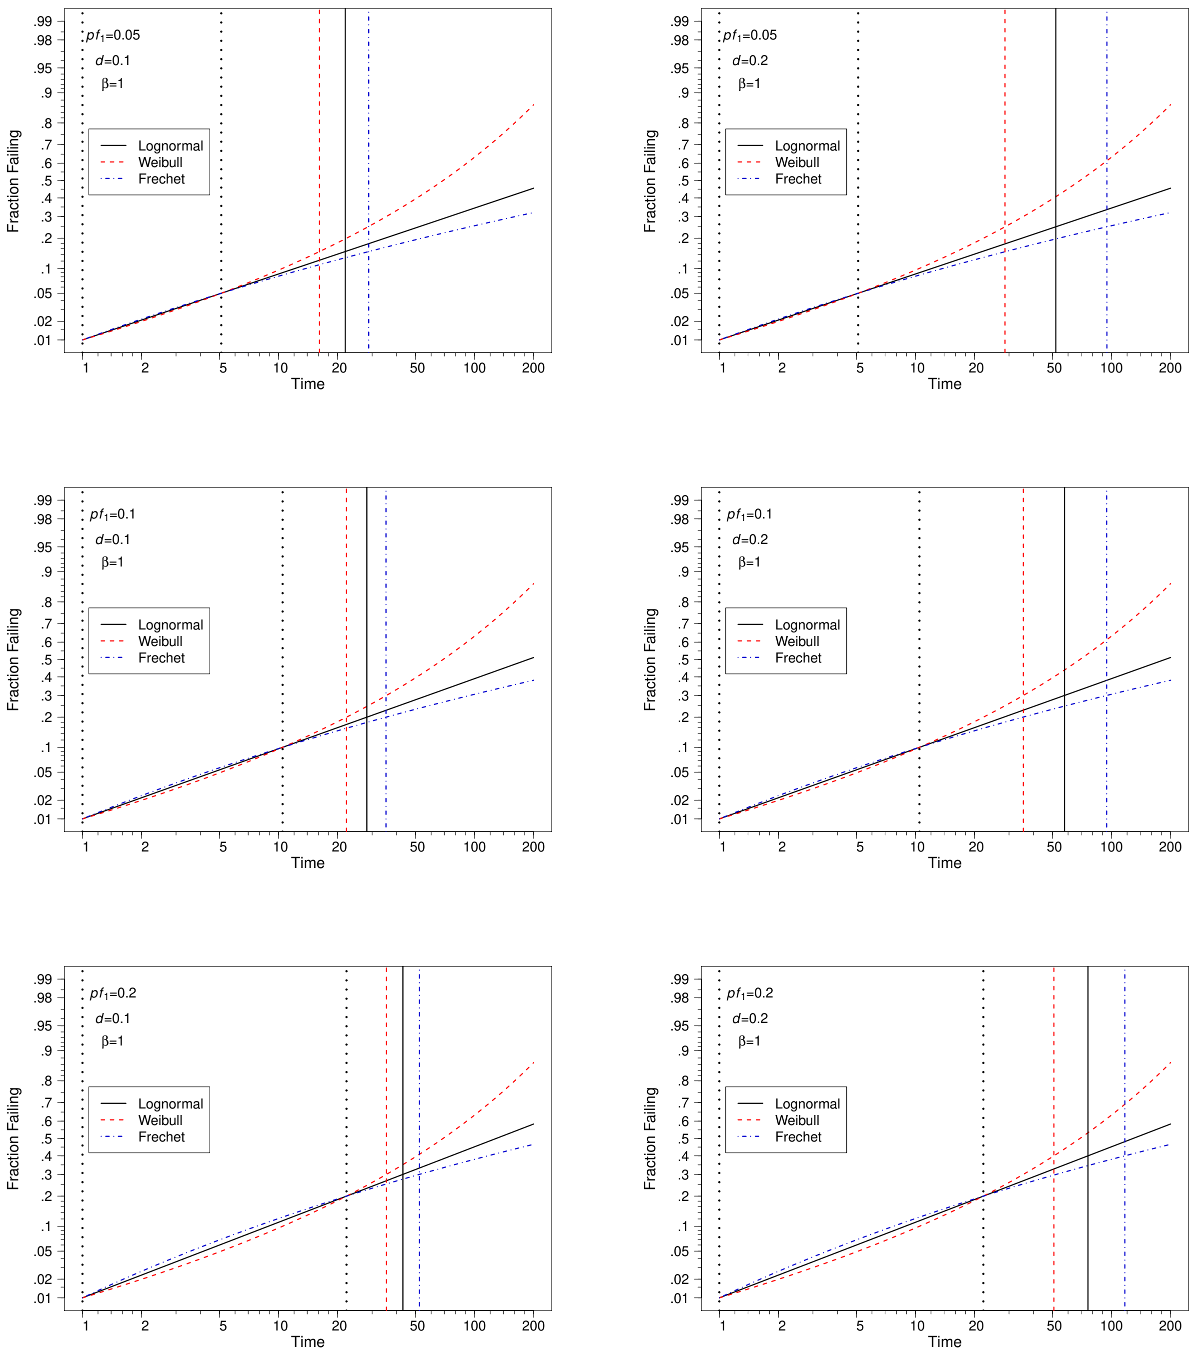


Figure 13: Distributional comparisons for $\beta = 1$. The two vertical dotted lines on the left indicate the points in time where all three distributions have the same 0.01 and $p_{f1}$ quantiles. The three vertical lines on the right indicate the times at $p_{f2} = p_{f1} + d$ for three distributions.

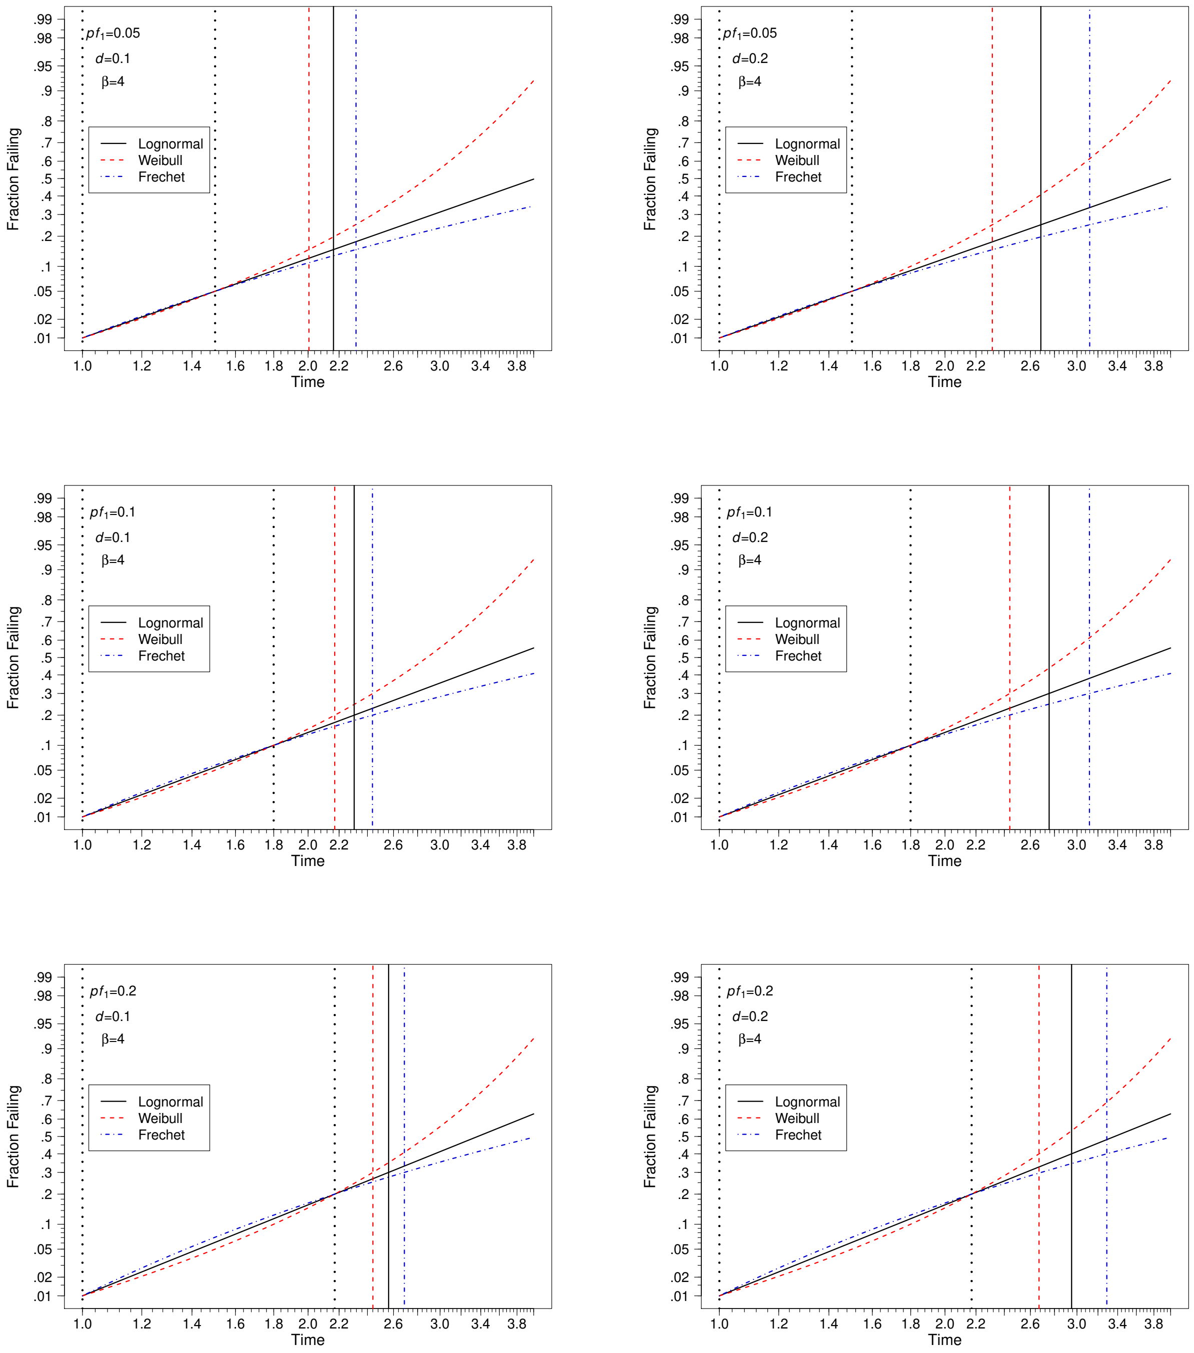


Figure 14: Distributional comparisons for $\beta = 4$. The two vertical dotted lines on the left indicate the points in time where all three distributions have the same 0.01 and $p_{f1}$ quantiles. The three vertical lines on the right indicate the times at $p_{f2} = p_{f1} + d$ for three distributions.
